# Supplementary material for: A Variational Approach for Joint Image Recovery and Feature Extraction Based on Spatially-Varying Generalised Gaussian Models
Source: arXiv:2209.01375 source file (2024-03-05)
Supplement: Supplementary file 2 [file supplement.pdf]

# Supplementary Material: A Variational Approach for Joint Image Recovery and Feature Extraction Based on Spatially Varying Generalised Gaussian Models

Émilie Chouzenoux<sup>1</sup>, Marie-Caroline Corbineau<sup>2</sup>, Jean-Christophe Pesquet<sup>1</sup>,  
Gabriele Scrivanti<sup>1\*</sup>

<sup>1</sup>Université Paris-Saclay, Inria, CentraleSupélec, CVN, France.

<sup>2</sup>Research department, Preligens, France.

\*Corresponding author(s). E-mail(s): [gabriele.scrivanti@centralesupelec.fr](mailto:gabriele.scrivanti@centralesupelec.fr);

## 1 Wavelet-based restoration

We illustrate the performance of our approach in the context of wavelet-based image restoration. The sought solution  $x \in \mathbb{R}^n$  corresponds to the wavelet coefficients of a source image  $\bar{x}$ , *i.e.*  $\bar{x} = Wx$  where  $W : \mathbb{R}^n \rightarrow \mathbb{R}^n$  models the Db8 wavelet orthogonal transform with 4 decomposition levels [1]. We choose  $\bar{x} \in [0, 255]^n$  to be the image *Westconcord* illustrated in Figure 1(a) and set  $H \in \mathbb{R}^{n \times n}$  as the blur operator modelling the convolution, using zero padding, with a  $11 \times 11$  Gaussian Kernel with zero-mean and standard deviation  $\sigma_b \in \{1.5, 2\}$ , which generates the blurred images  $H\bar{x} \in \mathbb{R}^n$  illustrated in Figure 1(b) and Figure 1(e). Hence, in this example, the linear operator in (1) corresponds to  $K = HW$ . Finally, we generate four noisy observation  $y \in \mathbb{R}^{n \times n}$  by applying model (1) using zero-mean Gaussian noise with standard deviation  $\sigma = 5$  (Figure 1(c) and Figure 1(f)) and  $\sigma = 10$  (Figure 1(d) and Figure 1(g)).

In this context we set  $[a, b] = [10^{-3}, 10]$ . We initialise the algorithm with  $x^0 = W^\top y$  that is the wavelet decomposition of the degraded image, while  $(p_i^0)_{1 \leq i \leq n}$  is drawn from an i.i.d. uniform distribution in the range  $[0.5, 1.5]$  and  $(\beta_i^0)_{1 \leq i \leq n}$  is drawn from an i.i.d. Gaussian distribution with

mean  $\mu_\beta$  and unit standard deviation, and the choice  $\mu_\beta = 5$  will be soon discussed. No preconditioning is considered in this example, that is  $A_\ell = \mathbb{I}_m$  for every  $\ell = 1, 2, \dots$  until convergence.

For comparisons, we consider the following models.

- The LASSO regularisation model (LASSO)

$$\underset{x \in \mathbb{R}^n}{\text{minimise}} \quad \frac{1}{2\sigma^2} \|Kx - y\|^2 + \xi \|x\|_1, \quad (1)$$

where  $\xi > 0$  is a regularisation parameter that is chosen through a grid search for PSNR and SSIM. We address (1) by means of a Forward-Backward algorithm.

- The Adaptive Order Non-Convex  $\ell_p$ -norm regularization model (AONCLP) from [2]

$$\underset{x \in \mathbb{R}^n}{\text{minimise}} \quad \frac{1}{2\sigma^2} \|Kx - y\|^2 + \xi \sum_{i=1}^n |x_i|^{\varpi(x_i)} \quad (2)$$

with  $\varpi : \mathbb{R} \rightarrow \mathbb{R}$  defined as  $t \mapsto 1 / (1 + \exp(-0.51(\log(|t| - 1))))$  and  $\xi > 0$  is a regularisation parameter that is chosen through a grid search for PSNR and SSIM. We address (2) by means of a Split Augmented Lagrangian Shrinkage Algorithm as described in [2].

- The Generalised Multivariate Exponential Power (GMEP) regularisation model from [3]:

$$\begin{aligned} \underset{x \in \mathbb{R}^n}{\text{minimise}} \quad & \frac{1}{2\sigma^2} \|Kx - y\|^2 \\ & + \xi \sum_{m=1}^M \sum_{c=1}^{C_m} (\rho_m^{1/\chi_m} x_{m,c}^2 + \delta)^{\chi_m}, \quad (3) \end{aligned}$$

where  $M$  is the number of wavelet subbands (in our case  $M = 13$ ),  $C_m$  the number of elements of the  $m$ -th subband ( $\sum_{m=1}^M C_m = n$ ),  $\delta = 10^{-6}$ , and the parameters  $\{\rho_1, \dots, \rho_M\}$  and  $\{\chi_1, \dots, \chi_M\}$  are obtained with a maximum likelihood estimator, run on each subband, of a Wiener-filtered version of the observed image  $y$ . Finally,  $\xi > 0$  is a regularisation parameter that is chosen through a grid search for PSNR and SSIM. Problem (3) is addressed by means of the Majorize-Minimize Memory Gradient (3MG) algorithm [4, 5].

In Figure 2 we illustrate the restored images obtained by the four regularisation models on the four degraded versions of the *Westconcord* image. The proposed model generates solutions which are competitive with the ones obtained by GMEP, with less artefacts and less saturated values than the ones obtained with LASSO and AONCLP. The good performance of our model is also supported by the quantitative evaluation illustrated in Table 1 in terms of PSNR and SSIM.

For what concerns the convergence properties of the algorithm, Figure 3 illustrates the decay of the objective values over 500 iterations for the different combinations of  $(\sigma_b, \sigma)$ . To study the stability with respect to the initialisations, we considered 10 random sampling for  $p^0$  and  $\beta^0$ : the continuous lines in the plots represent the mean objective values at each iteration and the shaded area, highlighted in the zoomed region at the centre of the plot, corresponds to the confidence interval related to the standard deviation of the objective value at each iteration. Figure 4 illustrates on a logarithmic scale the relative distance from the iterates to the solution  $\|\zeta^\ell - \zeta^\infty\|/\|\zeta^\infty\|$ , showing the convergence of our algorithm.

Figure 5, Figure 6 and Figure 7 illustrate the procedure that we adopted to identify an optimal value of parameter  $\mu_\beta$  in combination with  $\lambda$

and  $\zeta$ , for the reconstruction of the *Westconcord* image: in these figures we show in different forms the PSNR and SSIM scores for all the combinations of  $(\lambda, \zeta) \in \{0.01, 0.1, 1, 10, 100, 1000\}^2$  and  $\mu_\beta \in \{0, 2, 5, 7, 10\}$ . In particular, Figure 5 and Figure 6 show the PSNR and SSIM scores respectively in the forms of matrices, where each row corresponds to a value of  $\lambda$  and each column to a value of  $\zeta$ . For every combination  $(\sigma_b, \sigma)$ , we used the same colour scale for all the values of  $\mu_\beta$ , in order to highlight the variability of the results with respect to the whole triplet  $(\lambda, \zeta, \mu_\beta)$ : it can be seen that the parameter having the highest impact on the quality of the solution is  $\mu_\beta$ , while the impact of  $\lambda$  and  $\beta$  is weaker, especially on the SSIM, in spite of the fact that the choice for those values spans over 6 orders of magnitude. This is further highlighted in Figure 7, where the data are illustrated in the form of boxplots (PSNR scores in the left column and SSIM scores in the right column): from these plots we also infer that  $\mu_\beta = 5$  is a stable and optimal choice.

To conclude, we illustrate the performance of our method on a second group of test images: *Galaxy* which is a test image included in Matlab, *Buildings* from [6], and *Skyscrapers* from [7]. In this case, we set the noise level  $\sigma = 10$  and blur level  $\sigma_b \in \{1.5, 2\}$ . Figure 8 displays the degraded images, along with the reconstructions obtained with LASSO, AONCLP, GMEP, and our model, while Tables 2 and 3 report the PSNR and SSIM scores, which again advocates for the use of the proposed model. We also report for each method and for each image, the average computational time over 10 simulations required to meet the stopping criteria  $\|\zeta^{\ell+1} - \zeta^\ell\|/\|\zeta^\ell\| < 10^{-4}$  and  $|\theta(\zeta^{\ell+1}) - \theta(\zeta^\ell)|/|\theta(\zeta^\ell)| < 10^{-4}$ . Simulations were run on Matlab 2021b on an Intel Xeon Gold 6230 CPU 2.10GHz. A Matlab profiling of the simulations showed that the most time-consuming step is the update in (87), which is based on Newton's method. A possible solution to accelerate this step could consist in pre-computing a sufficiently large sample of solutions and replacing the computation with an indexing operation with respect to a lookup table.

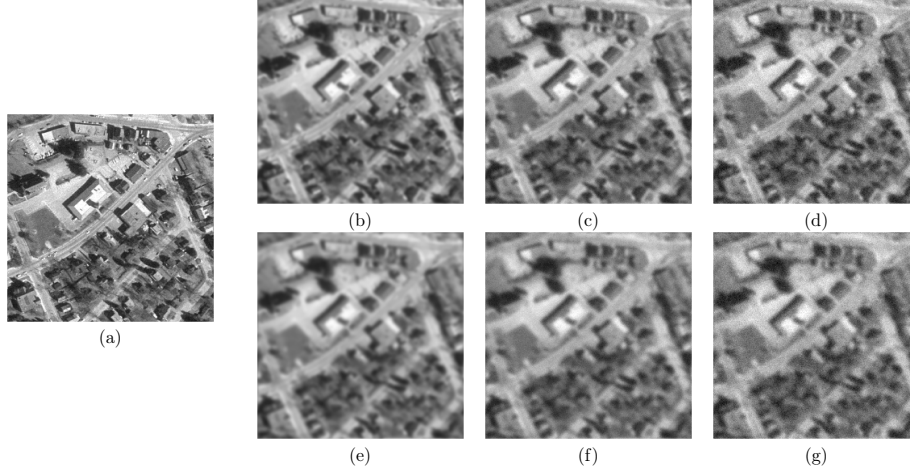

**Fig. 1:** *Westconcord* image: (a) original image, (b) blurred image with  $\sigma_b = 1.5$ , (c) degraded image with  $(\sigma_b, \sigma) = (1.5, 5)$  (PSNR = 22.49, SSIM = 0.55), (d) degraded image with  $(\sigma_b, \sigma) = (1.5, 10)$  (PSNR = 22.18, SSIM = 0.49); (e) blurred image with  $\sigma_b = 2$ , (f) degraded image with  $(\sigma_b, \sigma) = (2, 5)$  (PSNR = 21.07, SSIM = 0.43), (g) degraded image with  $(\sigma_b, \sigma) = (2, 10)$  (PSNR = 21.01, SSIM = 0.38).

| METHOD | $\sigma_b = 1.5$ |             |               |             | $\sigma_b = 2$ |             |               |             |
|--------|------------------|-------------|---------------|-------------|----------------|-------------|---------------|-------------|
|        | $\sigma = 5$     |             | $\sigma = 10$ |             | $\sigma = 5$   |             | $\sigma = 10$ |             |
|        | PSNR             | SSIM        | PSNR          | SSIM        | PSNR           | SSIM        | PSNR          | SSIM        |
| LASSO  | 24.48            | 0.66        | 23.33         | 0.58        | 23.65          | 0.59        | 22.62         | 0.50        |
| AONCLP | 24.32            | 0.64        | 23.29         | 0.56        | 22.87          | 0.54        | 22.56         | 0.49        |
| GMEP   | 24.61            | <b>0.68</b> | 23.91         | <b>0.63</b> | 22.94          | 0.57        | 22.70         | <b>0.54</b> |
| OURS   | <b>24.83</b>     | <b>0.68</b> | <b>24.27</b>  | 0.62        | <b>24.41</b>   | <b>0.60</b> | <b>24.42</b>  | 0.53        |

**Table 1:** PSNR and SSIM scores for *Westconcord* example.

## 2 Parameter Tuning for joint deblurring/segmentation

Figures 9-12 illustrate the procedure that we adopted to identify an optimal value of parameter  $\mu_\beta$  in combination with  $\lambda$  and  $\zeta$ , for the reconstruction of *Simu1* and *Simu2*. In these figures, for all the combinations of  $(\lambda, \zeta) \in \{0.01, 0.1, 1, 10, 100, 1000\}^2$  and  $\mu_\beta \in \{-5, -2, 0, 2, 5\}$  for *Simu1* and  $\mu_\beta \in \{0, 2, 3, 4, 5\}$  for *Simu2*, we show in different forms the PSNR and SSIM scores for the reconstruction of the images, while for the shape parameter we rely on the RMSE the OA of the segmentation. In particular, Figures 9 and 10 illustrate the results in the form of matrices, where each row corresponds to a value of  $\lambda$  and each column to a value of  $\zeta$ . Figures 11 and 12 illustrate the results in the form

of boxplots. The values of the PSNR and SSIM are mostly affected by the value of  $\mu_\beta$ , while less variability is related to the choice of  $\lambda$  and  $\zeta$ . On the other side, RMSE and OA depend on a combination of the three parameters (in particular on a combination of  $\mu_\beta$  and  $\lambda$ ). In conclusion, for the choice of  $\mu_\beta$ , we relied on the value that could provide us with the best trade-off between high PSNR/SSIM, high OA and low RMSE. For *Simu1*, this choice is clearly represented by  $\mu_\beta = 0$ , as with this value we manage to optimise all the metrics. For *Simu2*, the best trade-off is represented by  $\mu_\beta = 4$ , as  $\mu_\beta = 5$  yields high PSNR/SSIM levels on one side, but unsatisfactory OA and RMSE on the other.

| $(\sigma_b, \sigma)$ | DEGRADED | LASSO | AONCLP | GMEP | OURS |
|----------------------|----------|-------|--------|------|------|
| $(1.5, 5)$           |          |       |        |      |      |
| $(1.5, 10)$          |          |       |        |      |      |
| $(2, 5)$             |          |       |        |      |      |
| $(2, 10)$            |          |       |        |      |      |

**Fig. 2:** Estimated solutions for *Westconcord* image. First column: Degraded image. Second column: LASSO regularisation. Third column: AONCLP regularisation. Fourth column: GMEP regularisation. Fifth column: Proposed regularisation.

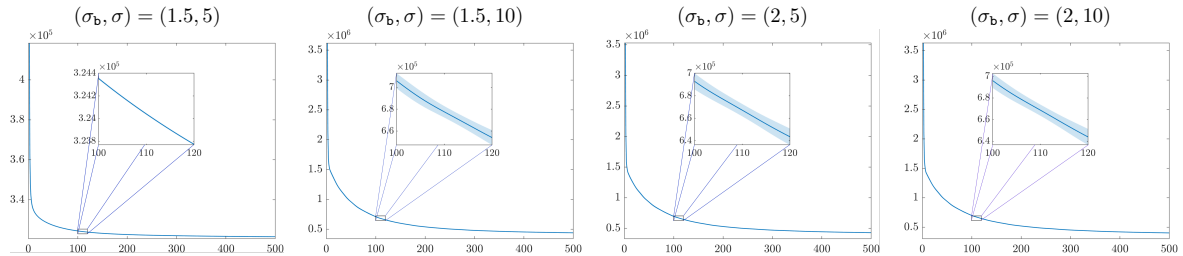

**Fig. 3:** Decay of the objective value along 500 iterations for *Westconcord* example, using different combinations of  $(\sigma_b, \sigma)$ . We considered 10 random sampling for  $p^0$  and  $\beta^0$ . The continuous line in the plot represents the mean objective value at each iteration and the shaded area, highlighted in the zoomed region at the centre of the plot spanning over 20 iterations, corresponds to the confidence interval related to the standard deviation.

## References

- [1] Daubechies, I., Sweldens, W.: Factoring wavelet transforms into lifting steps. *Journal of Fourier Analysis and Applications* **4**, 247–269 (1998)
- [2] Afonso, M., Sanches, J.M.: Adaptive order non-convex lp-norm regularization in image restoration. *Journal of Physics: Conference Series* **904**(1), 012016 (2017)
- [3] Marnissi, Y., Benazza-Benyahia, A.,



| METHOD | <i>Galaxy</i> |             |       | <i>Buildings</i> |             |       | <i>Skyscrapers</i> |             |       |
|--------|---------------|-------------|-------|------------------|-------------|-------|--------------------|-------------|-------|
|        | PSNR          | SSIM        | TIME  | PSNR             | SSIM        | TIME  | PSNR               | SSIM        | TIME  |
| LASSO  | 25.25         | 0.34        | 42.8  | 24.35            | 0.38        | 34.2  | 21.57              | 0.32        | 30.8  |
| AONCLP | 25.15         | 0.32        | 21.4  | 24.08            | 0.37        | 24.5  | 21.70              | 0.31        | 42.4  |
| GMEP   | <b>25.75</b>  | 0.37        | 12.7  | 24.45            | 0.38        | 14.1  | 21.43              | 0.33        | 13.78 |
| OURS   | 25.12         | <b>0.37</b> | 219.7 | <b>25.23</b>     | <b>0.40</b> | 441.5 | <b>21.88</b>       | <b>0.33</b> | 405.9 |

**Table 2:** PSNR scores, SSIM scores, and computational times (in seconds) for  $(\sigma_b, \sigma) = (1.5, 10)$ .

| METHOD | <i>Galaxy</i> |             |       | <i>Buildings</i> |             |       | <i>Skyscrapers</i> |             |       |
|--------|---------------|-------------|-------|------------------|-------------|-------|--------------------|-------------|-------|
|        | PSNR          | SSIM        | TIME  | PSNR             | SSIM        | TIME  | PSNR               | SSIM        | TIME  |
| LASSO  | 24.72         | 0.28        | 43.7  | 23.12            | 0.29        | 35.1  | 20.91              | 0.24        | 35.1  |
| AONCLP | 24.66         | 0.28        | 15.0  | 23.20            | 0.29        | 27.4  | 20.79              | 0.24        | 27.4  |
| GMEP   | 24.98         | 0.30        | 12.2  | 23.30            | 0.30        | 10.9  | 20.35              | 0.25        | 10.9  |
| OURS   | <b>25.08</b>  | <b>0.32</b> | 329.1 | <b>24.92</b>     | <b>0.30</b> | 766.4 | <b>21.53</b>       | <b>0.25</b> | 379.1 |

**Table 3:** PSNR scores, SSIM scores and computational times (in seconds) for  $(\sigma_b, \sigma) = (2, 10)$ .

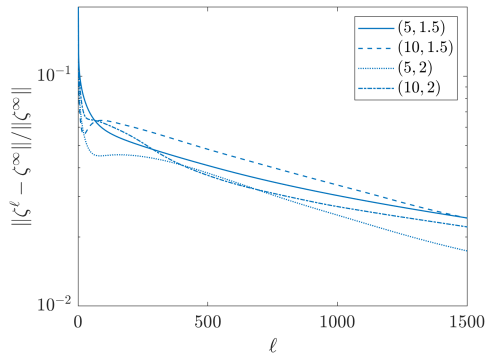

**Fig. 4:** Convergence plots for four settings of  $(\sigma_b, \sigma)$ , in terms of distance from the iterates  $\zeta^\ell$  to the solution  $\zeta^\infty$ , for *Westconcord* example.

Chouzenoux, E., Pesquet, J.-C.: Generalized multivariate exponential power prior for wavelet-based multichannel image restoration. In: 2013 IEEE International Conference on Image Processing, pp. 2402–2406 (2013). <https://doi.org/10.1109/ICIP.2013.6738495>

- [4] Chouzenoux, E., Idier, J., Moussaoui, S.: A majorize–minimize strategy for subspace optimization applied to image restoration. *IEEE Transactions on Image Processing* **20**(6), 1517–1528 (2011)

- [5] Chouzenoux, E., Jezierska, A., Pesquet, J.-C., Talbot, H.: A majorize–minimize subspace approach for  $\ell_2 - \ell_0$  image regularization. *SIAM Journal on Imaging Sciences* **6**(1), 563–591 (2013)

- [6] Caesar, H., Uijlings, J., Ferrari, V.: Joint calibration for semantic segmentation. In: *British Machine Vision Conference 2015*, p. 29 (2015). BMVA Press

- [7] Lanza, A., Morigi, S., Pragliola, M., Sgalari, F.: Space-variant generalised Gaussian regularisation for image restoration. *Computer Methods in Biomechanics and Biomedical Engineering: Imaging and Visualization* **7**, 1–14 (2018)

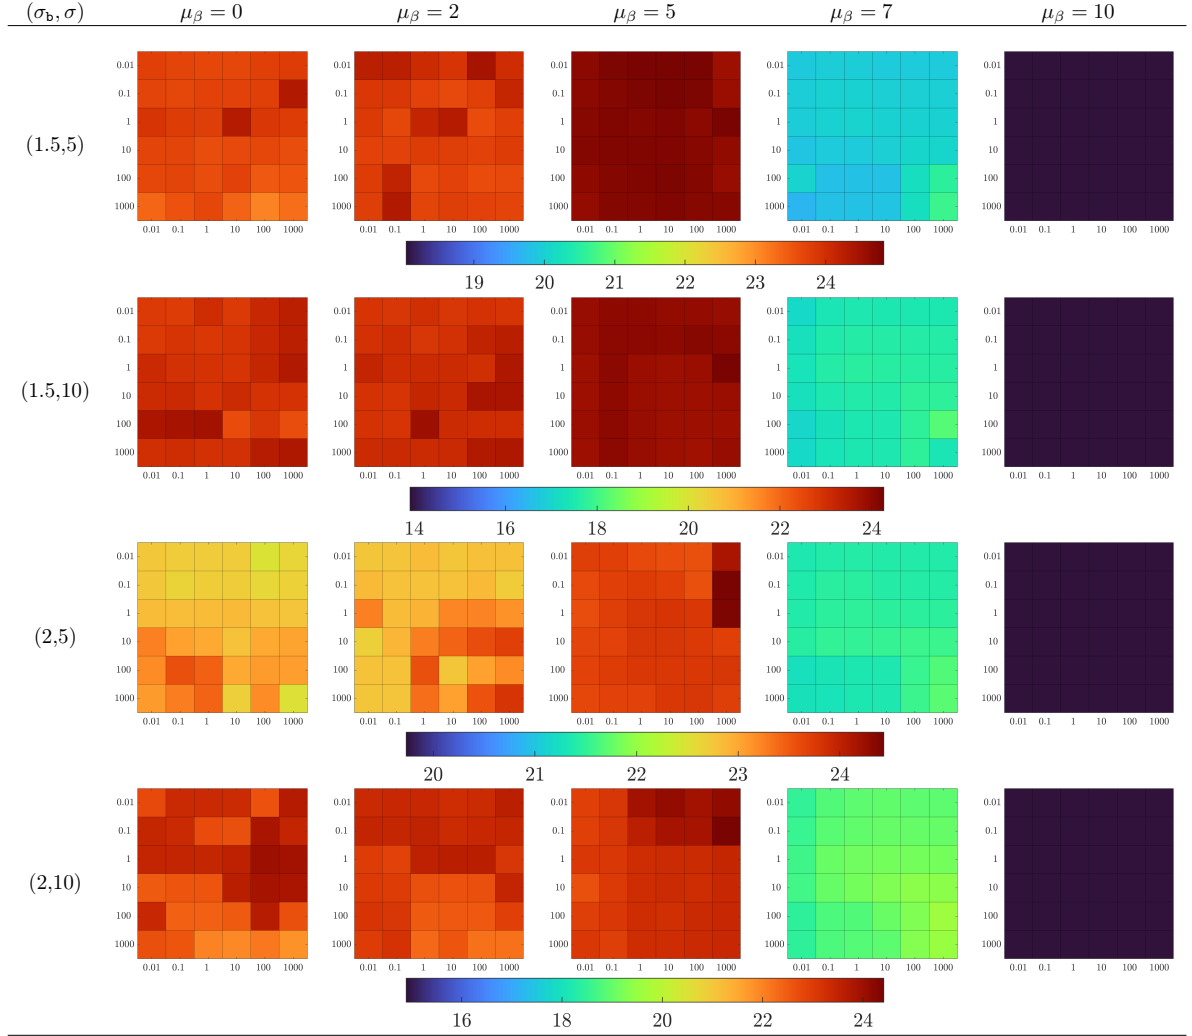

**Fig. 5:** Illustration of the PSNR scores obtained with a grid search on parameters  $(\lambda, \zeta)$  for *Westconcord* for 5 different choices for parameter  $\mu_\beta$ . In each matrix, rows correspond to the values for  $\lambda$  and columns to the values for  $\zeta$ . For each parameter we chose 6 values in a logarithmic scale between  $10^{-2}$  and  $10^3$ .

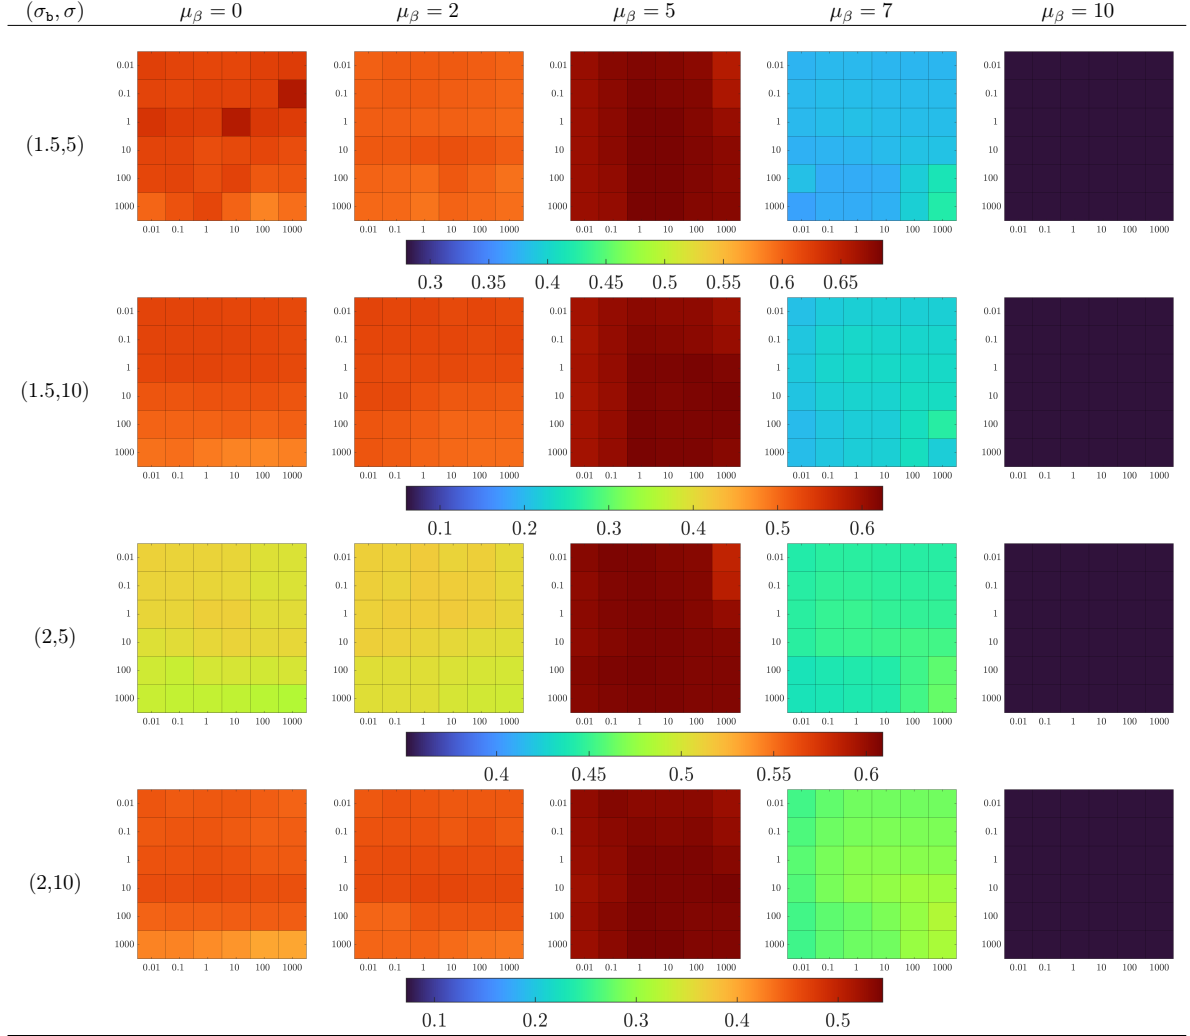

**Fig. 6:** Illustration of the SSIM scores obtained with a grid search on parameters  $(\lambda, \zeta)$  for *Westconcord* for 5 different choices for parameter  $\mu_\beta$ . In each matrix, rows correspond to the values for  $\lambda$  and columns to the values for  $\zeta$ . For each parameter we chose 6 values in a logarithmic scale between  $10^{-2}$  and  $10^3$ .

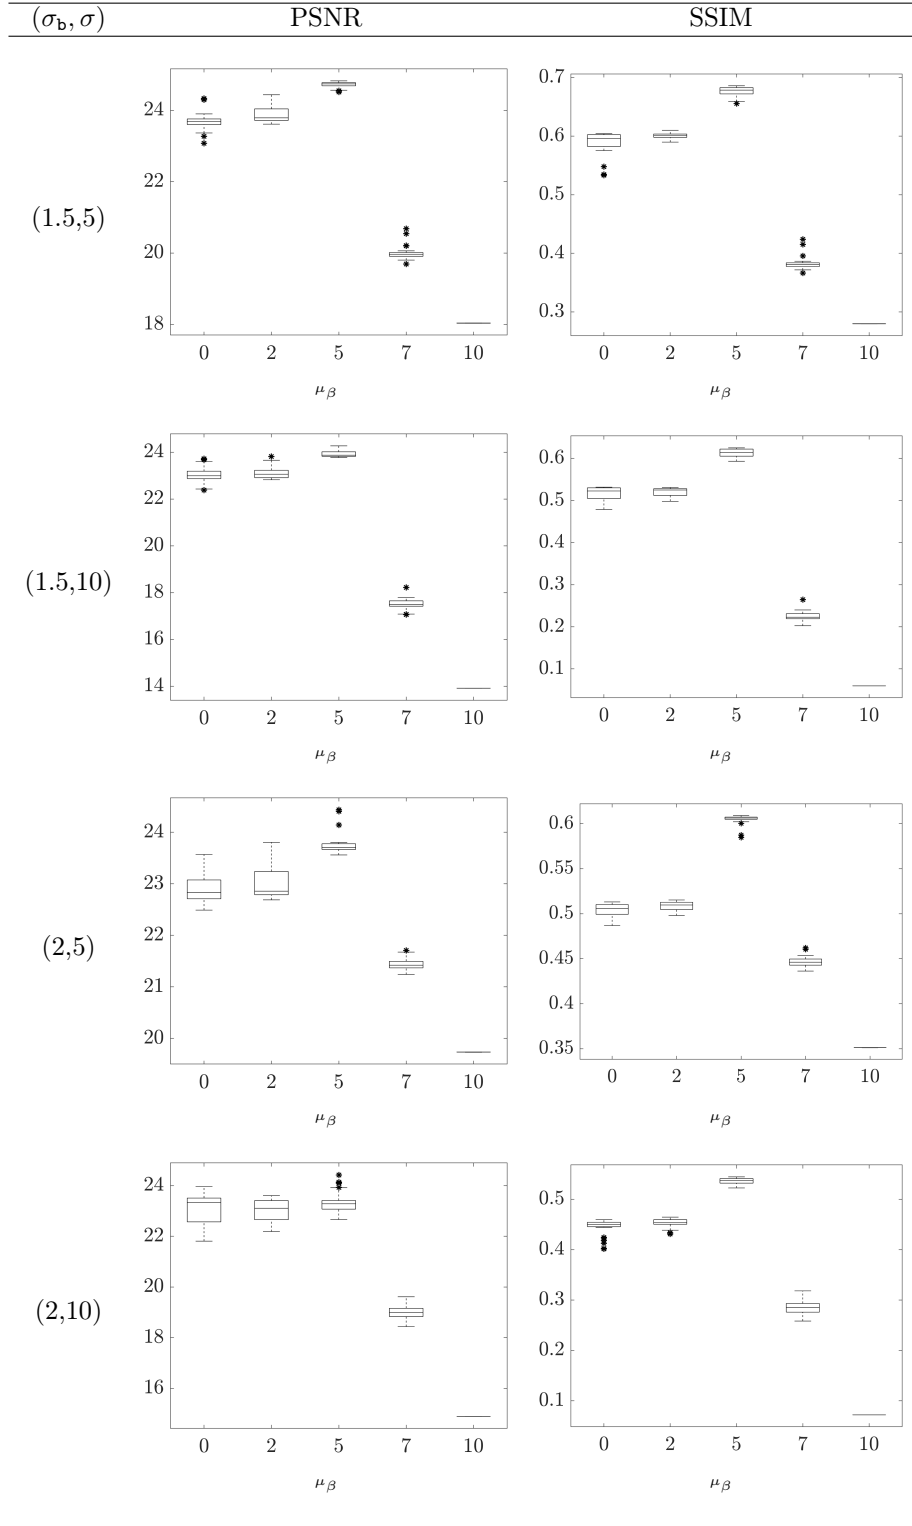

**Fig. 7:** Boxplots of the PSNR scores (left column) and SSIM scores (right column) obtained with a grid search on parameters  $(\lambda, \zeta)$  for *Westconcord* for 5 different choices for parameter  $\mu_\beta$ . The rows corresponds to different combinations of  $(\sigma_b, \sigma)$  with  $\sigma_b \in \{1.5, 2\}$  and  $\sigma \in \{5, 10\}$ .



| $\sigma_b$ | DEGRADED                                                                            | LASSO                                                                               | AONCLP                                                                              | GMEP                                                                                 | OURS                                                                                  |
|------------|-------------------------------------------------------------------------------------|-------------------------------------------------------------------------------------|-------------------------------------------------------------------------------------|--------------------------------------------------------------------------------------|---------------------------------------------------------------------------------------|
| 1.5        | 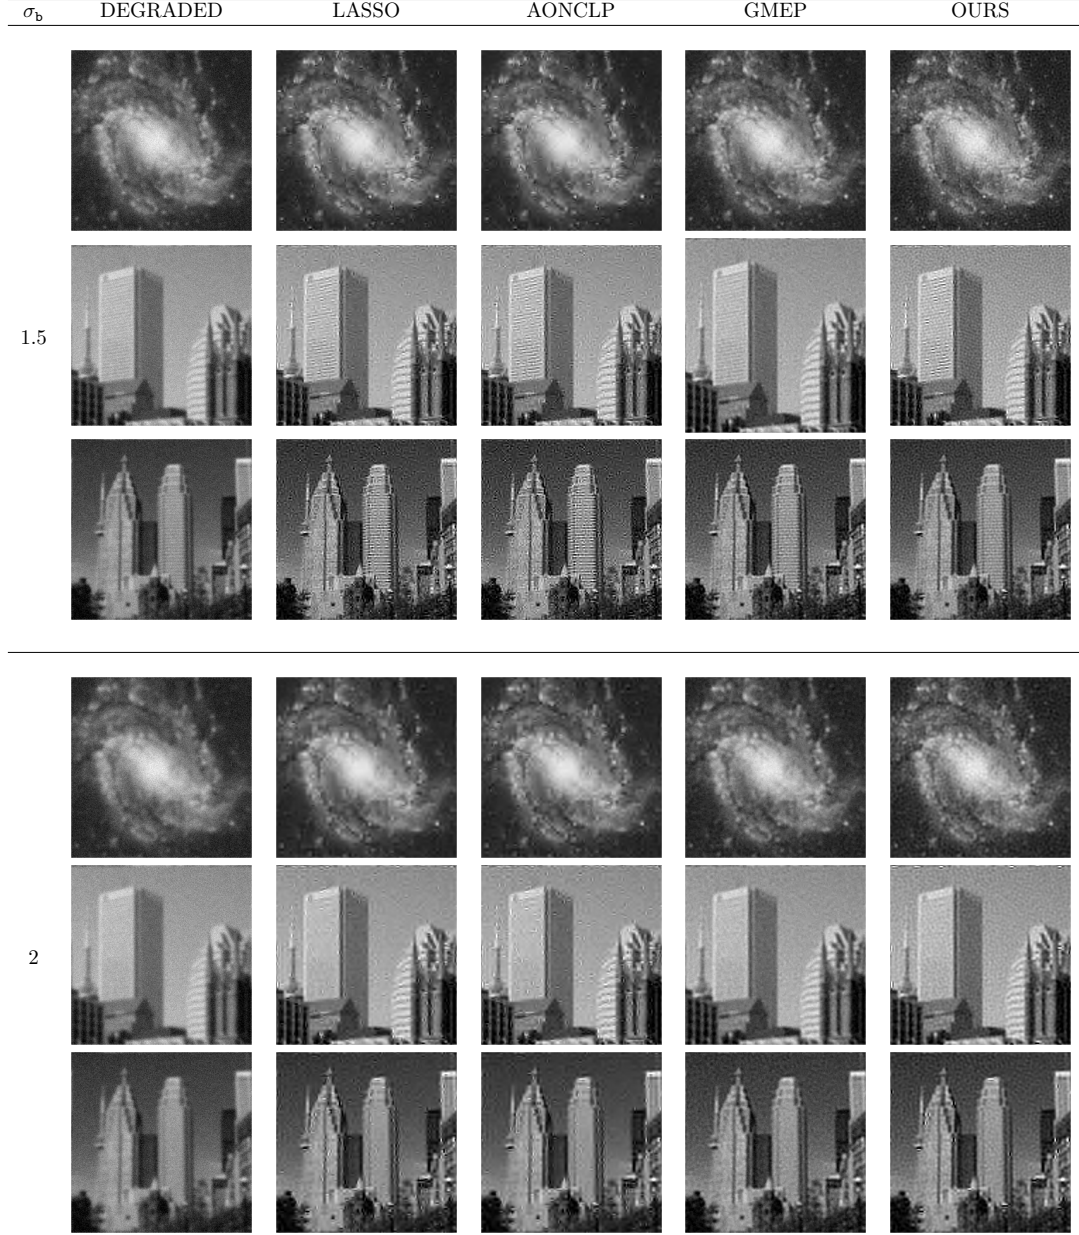   | 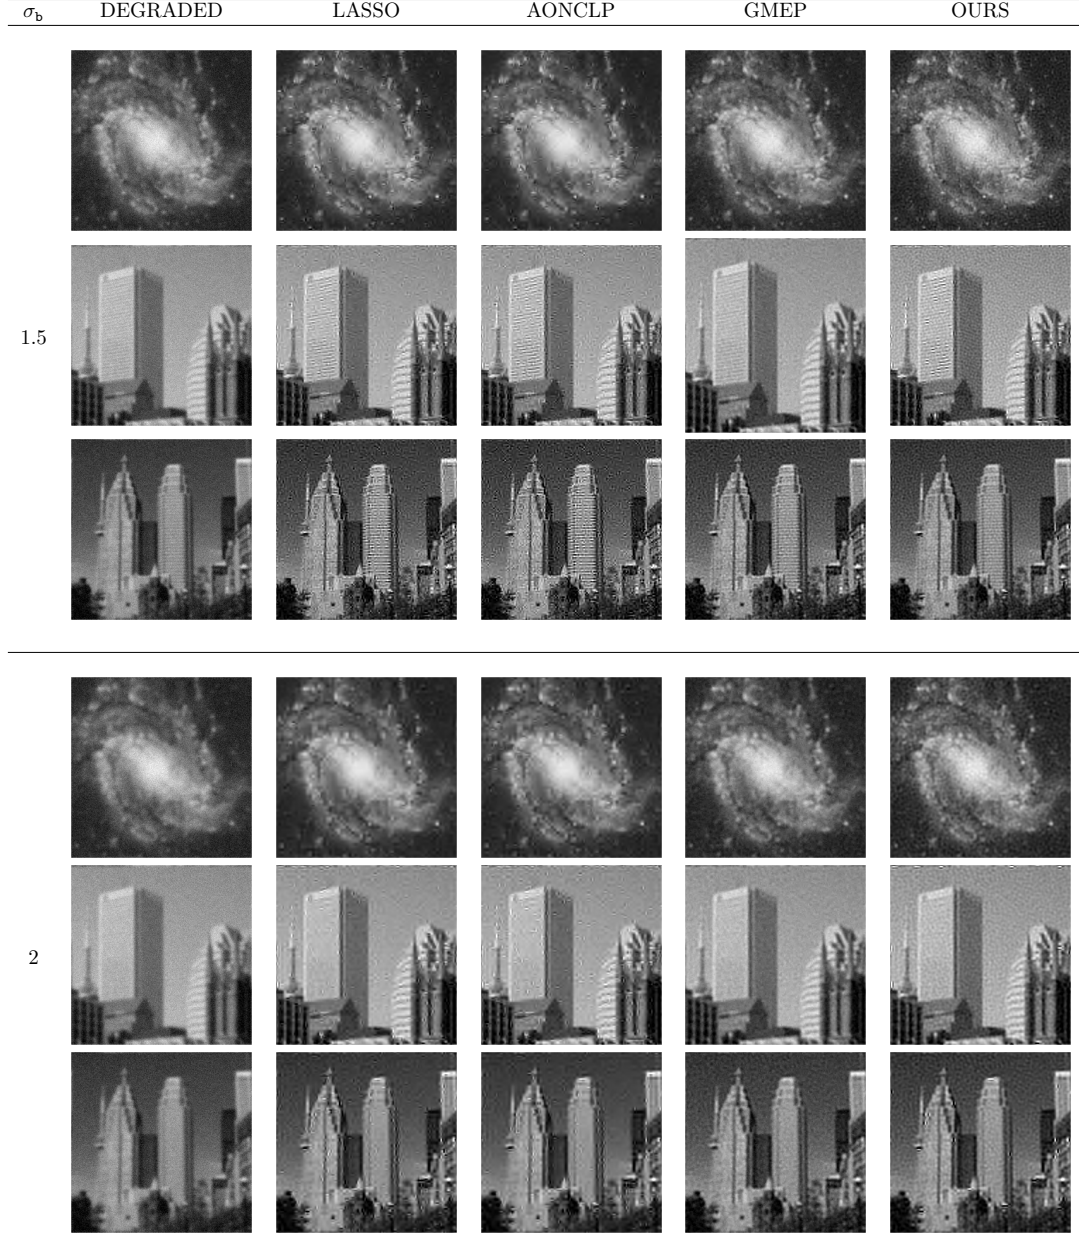   | 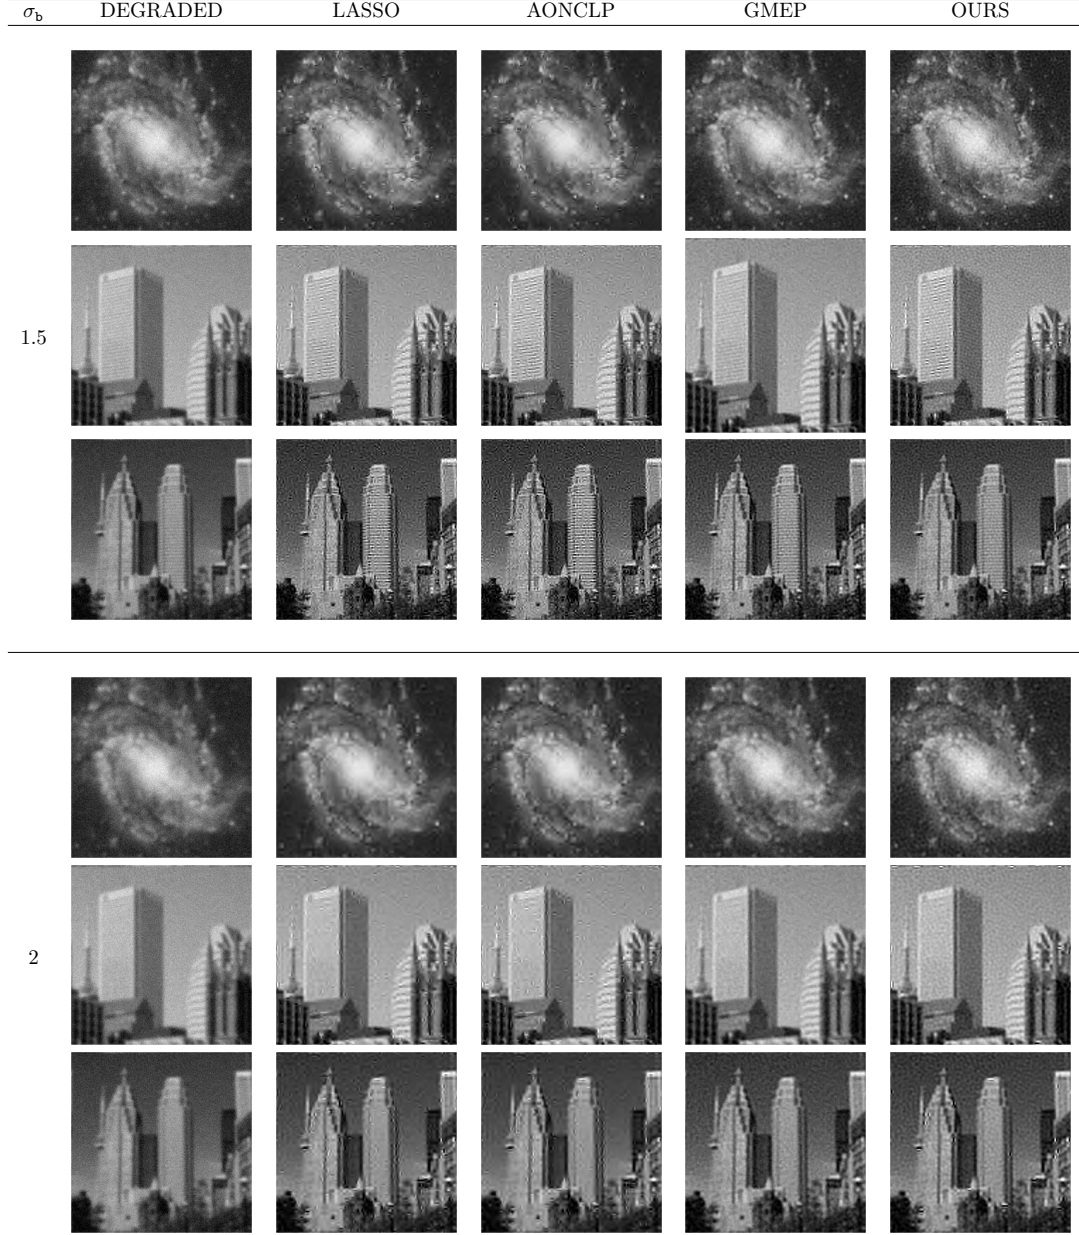   | 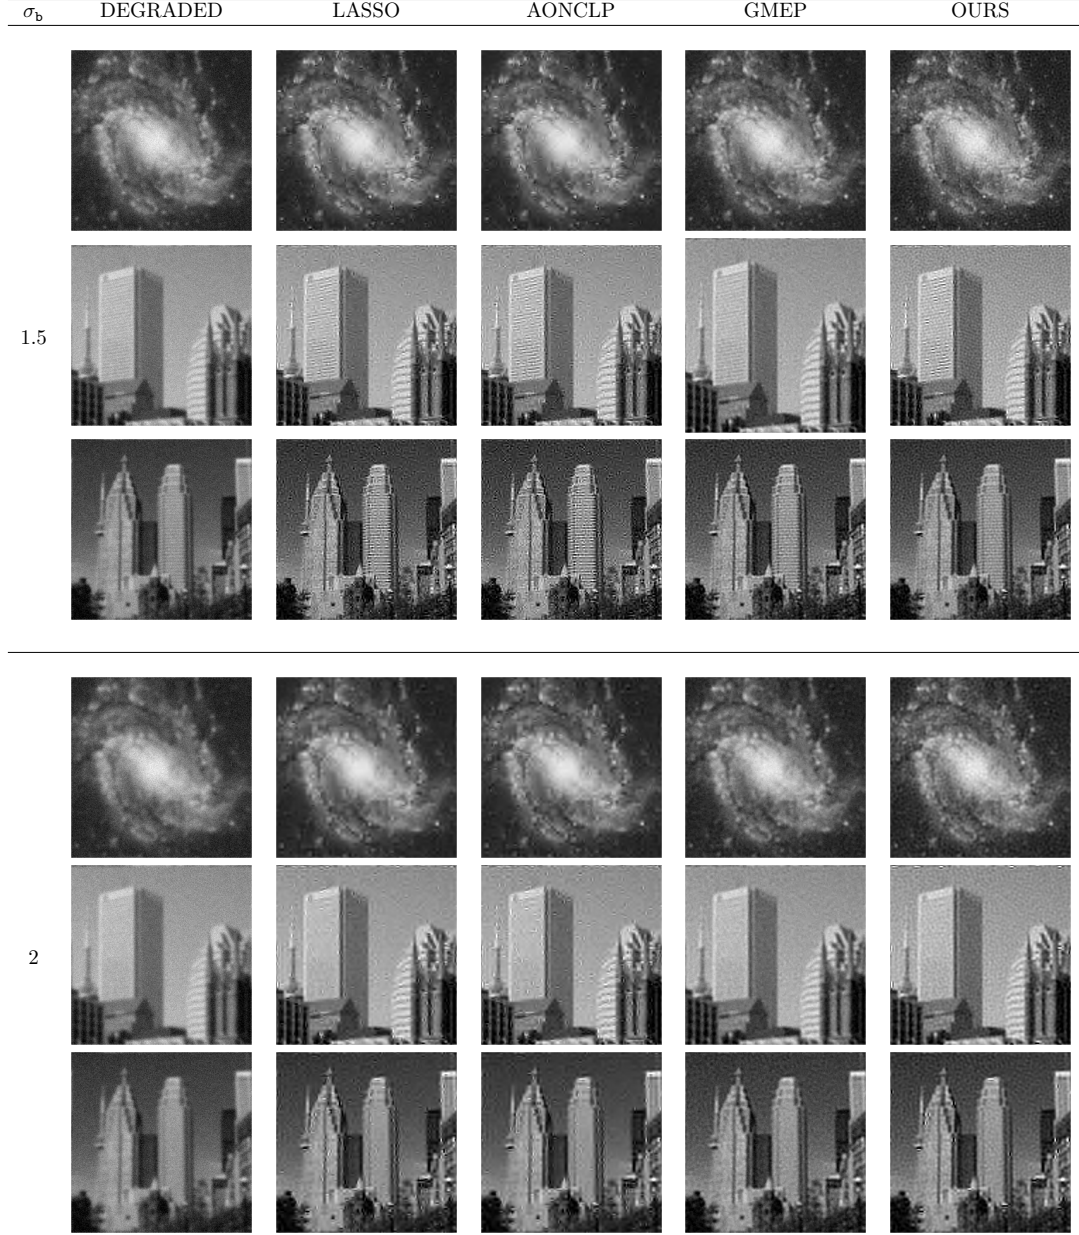   | 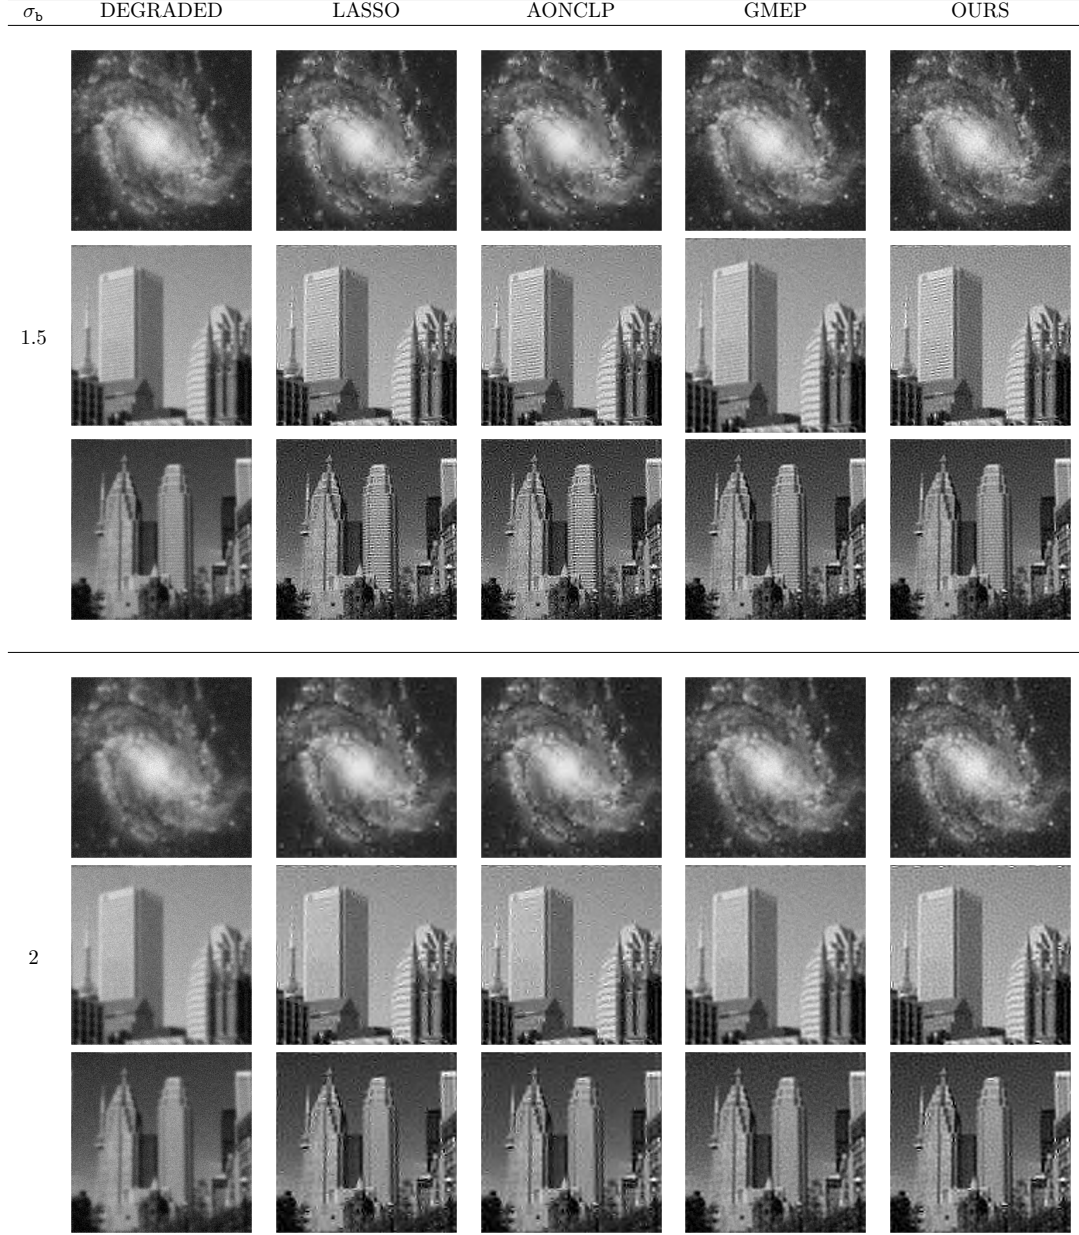   |
|            | 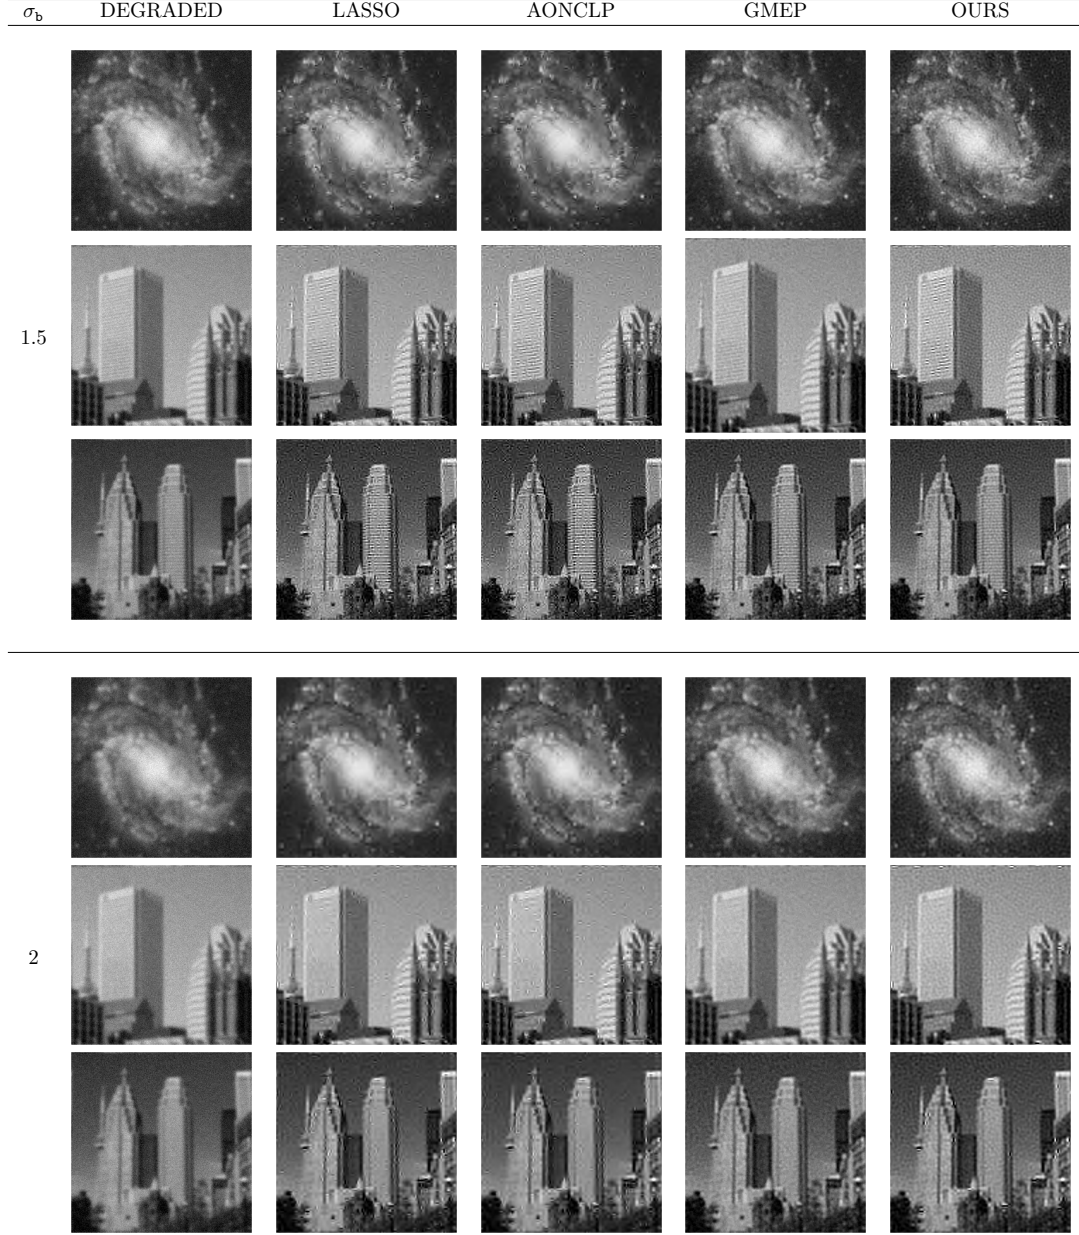   | 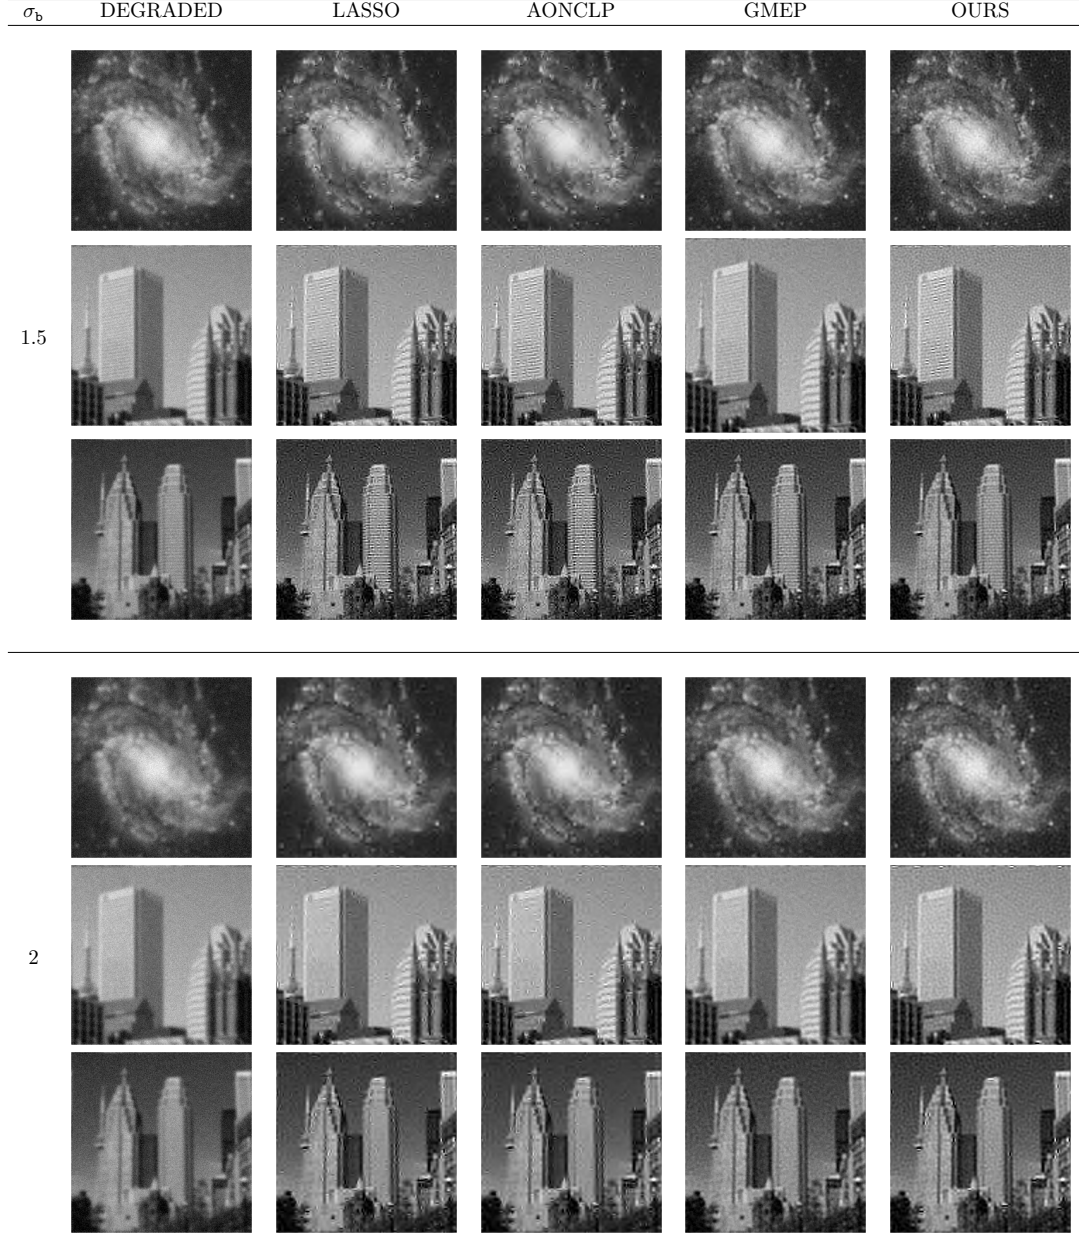   | 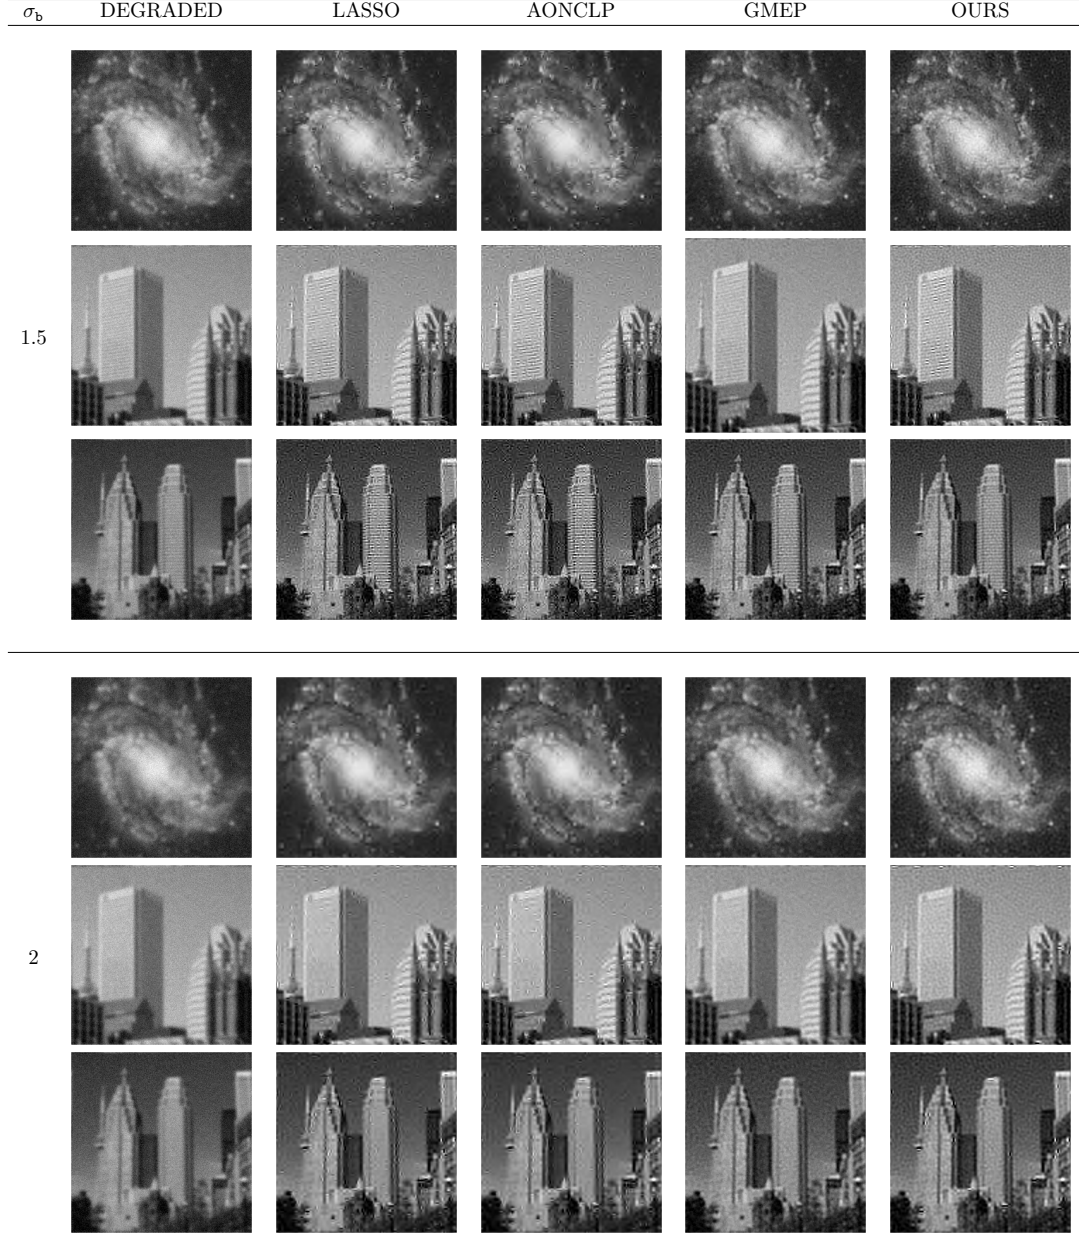   | 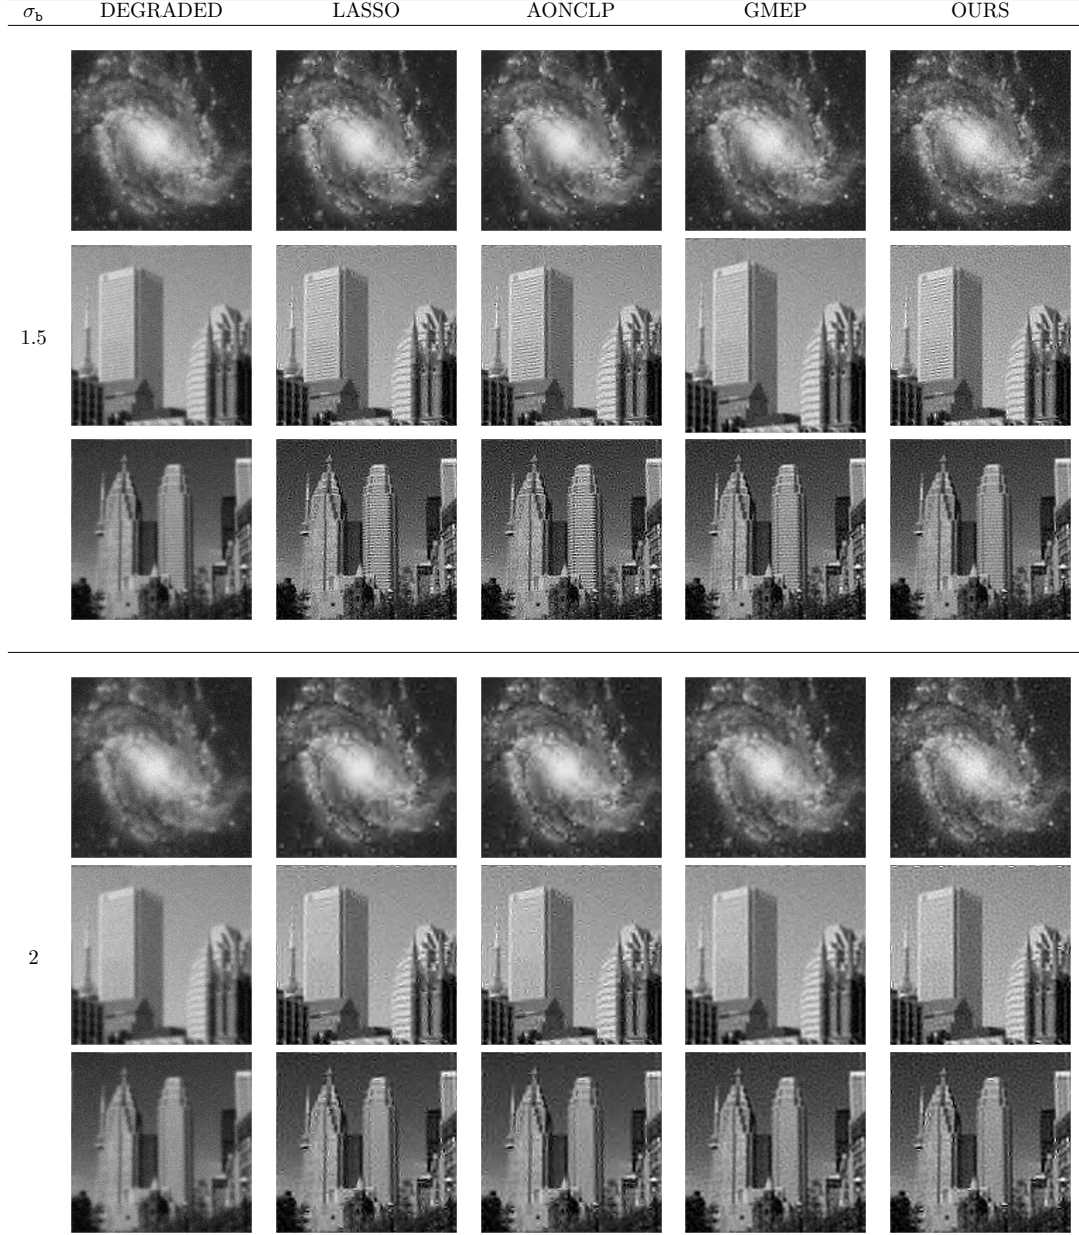   | 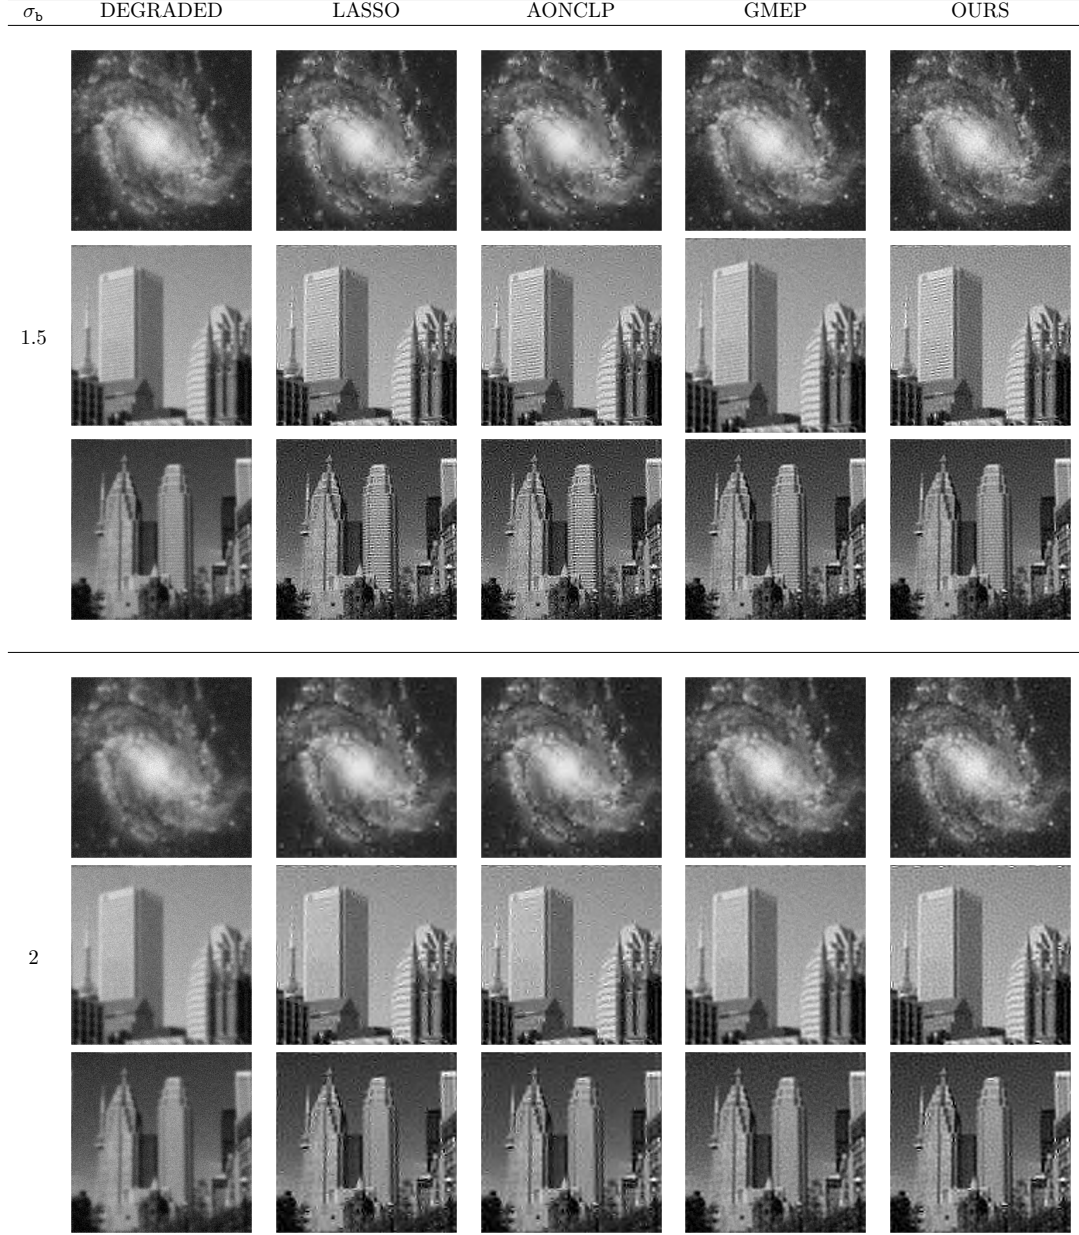   |
|            | 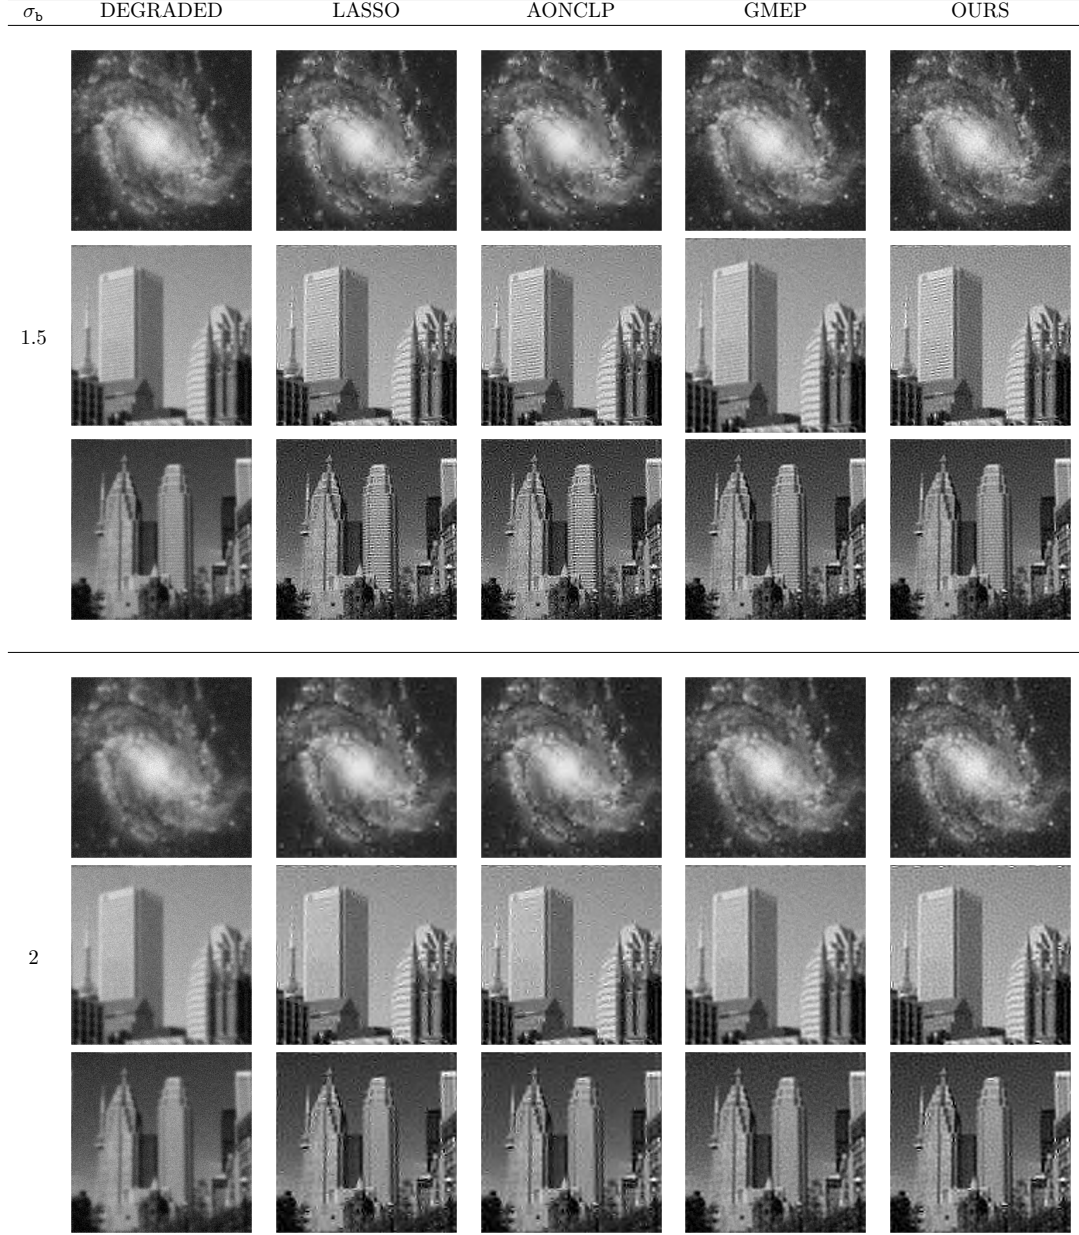   | 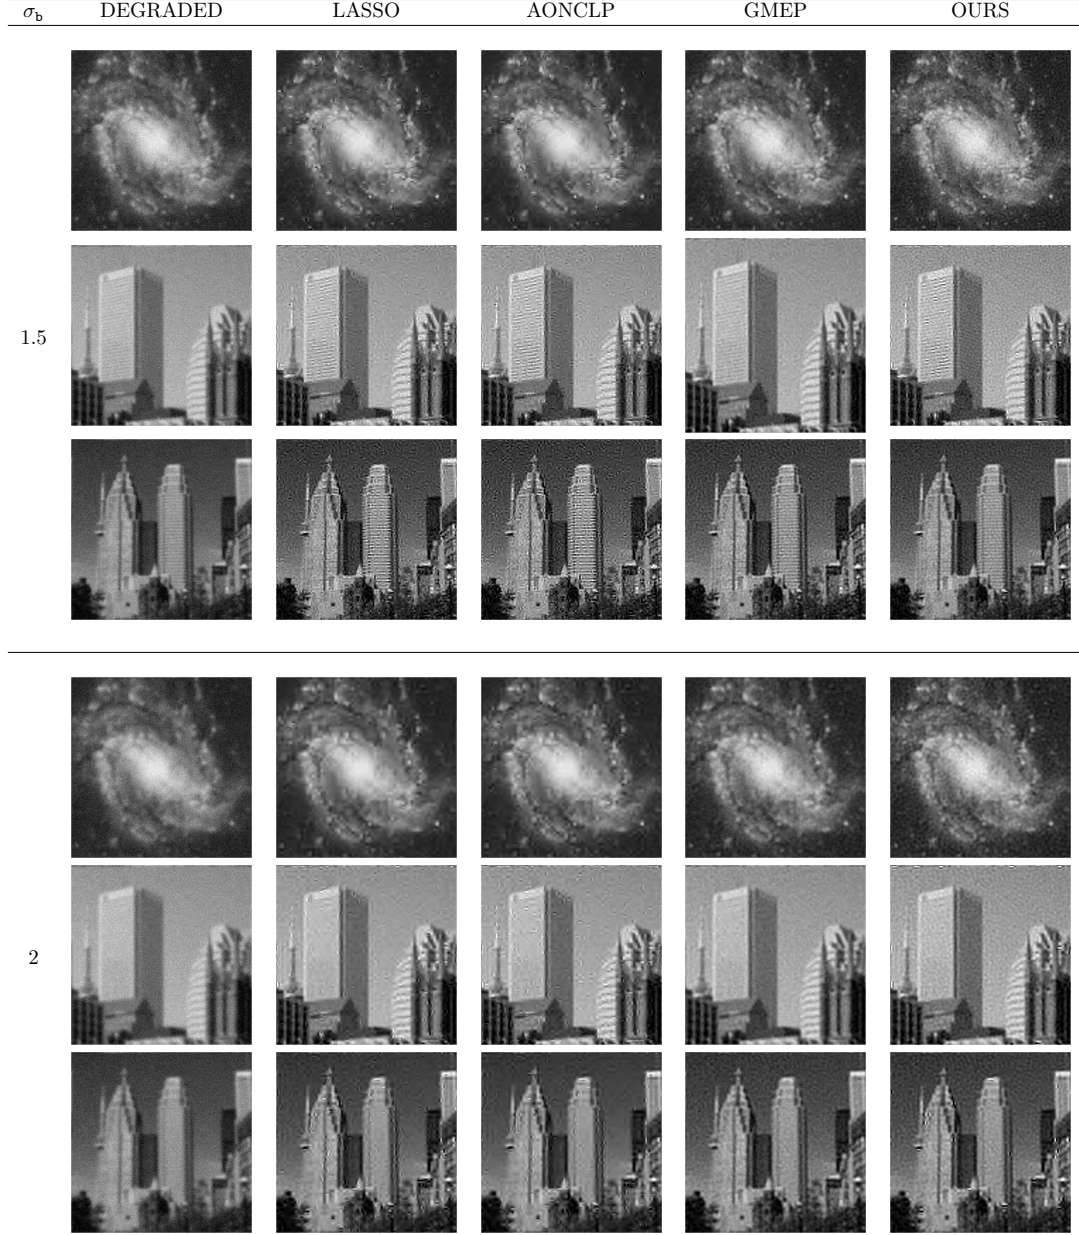   | 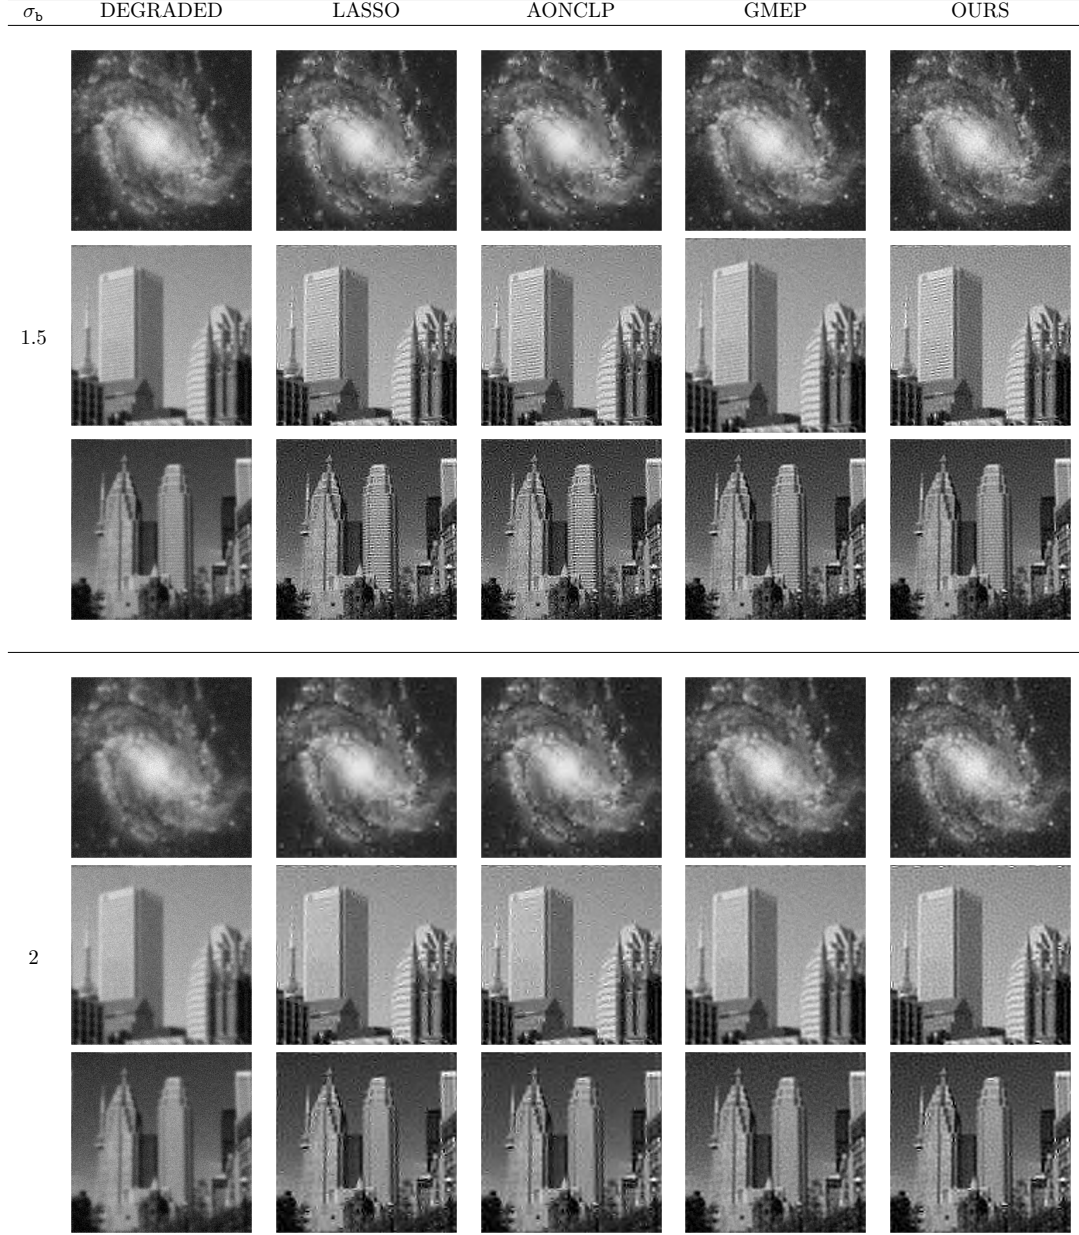   | 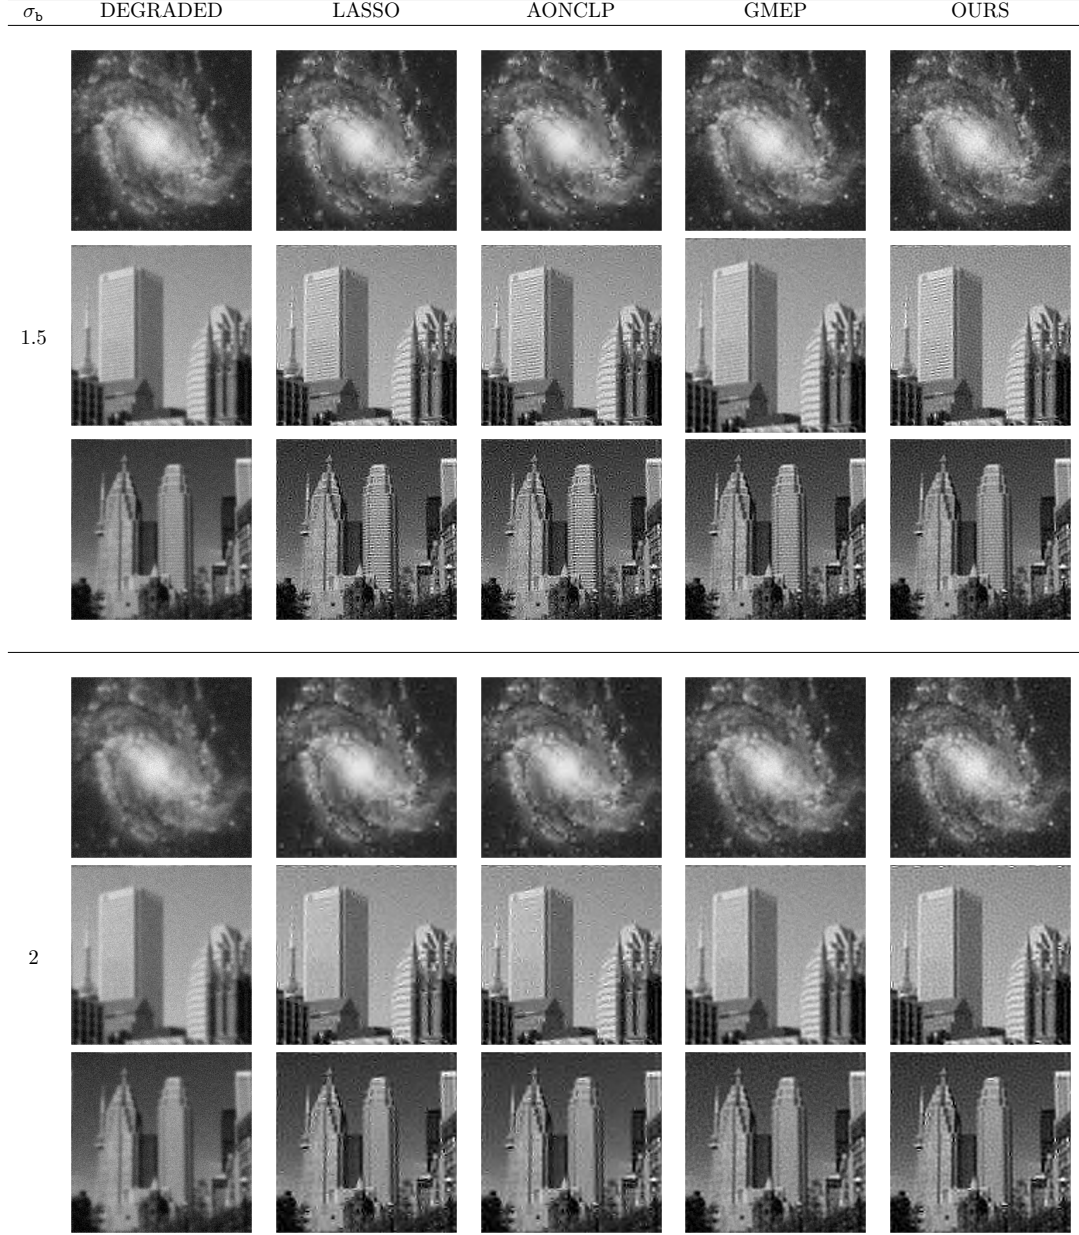   | 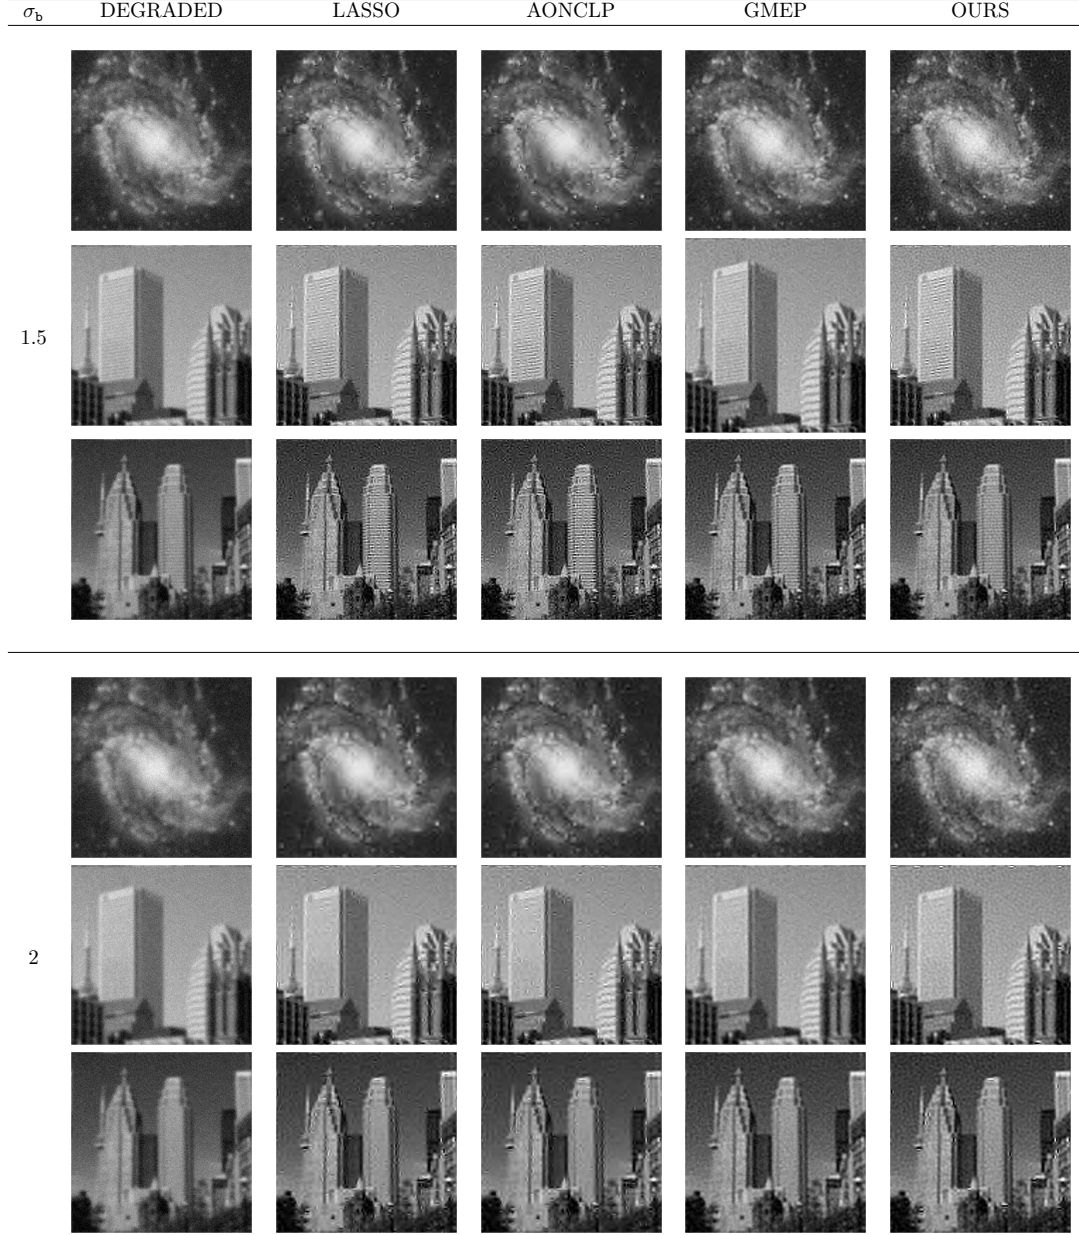   |
| 2          | 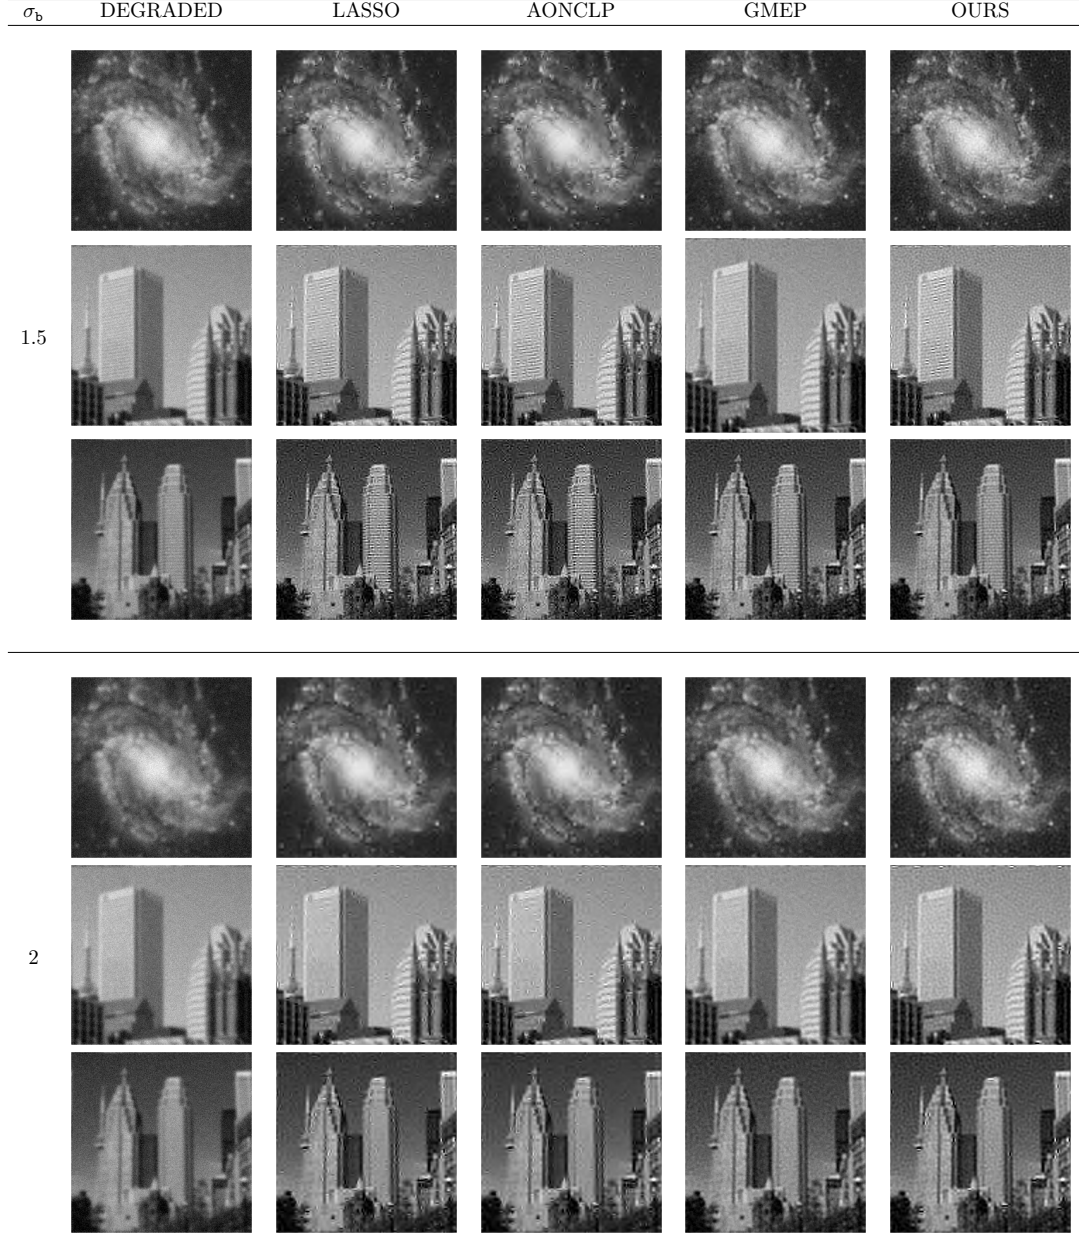  | 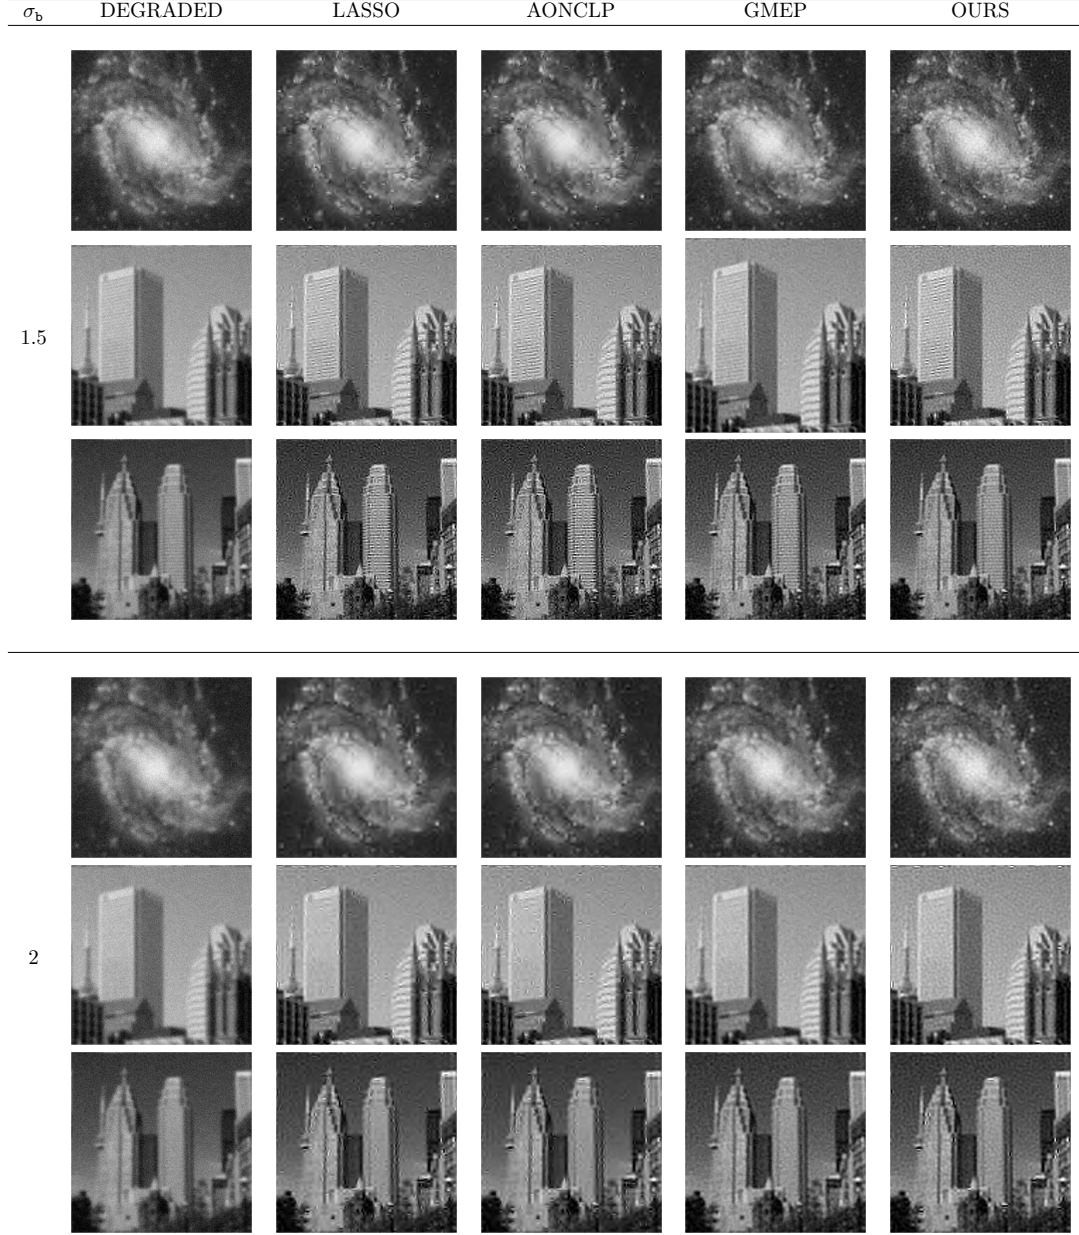  | 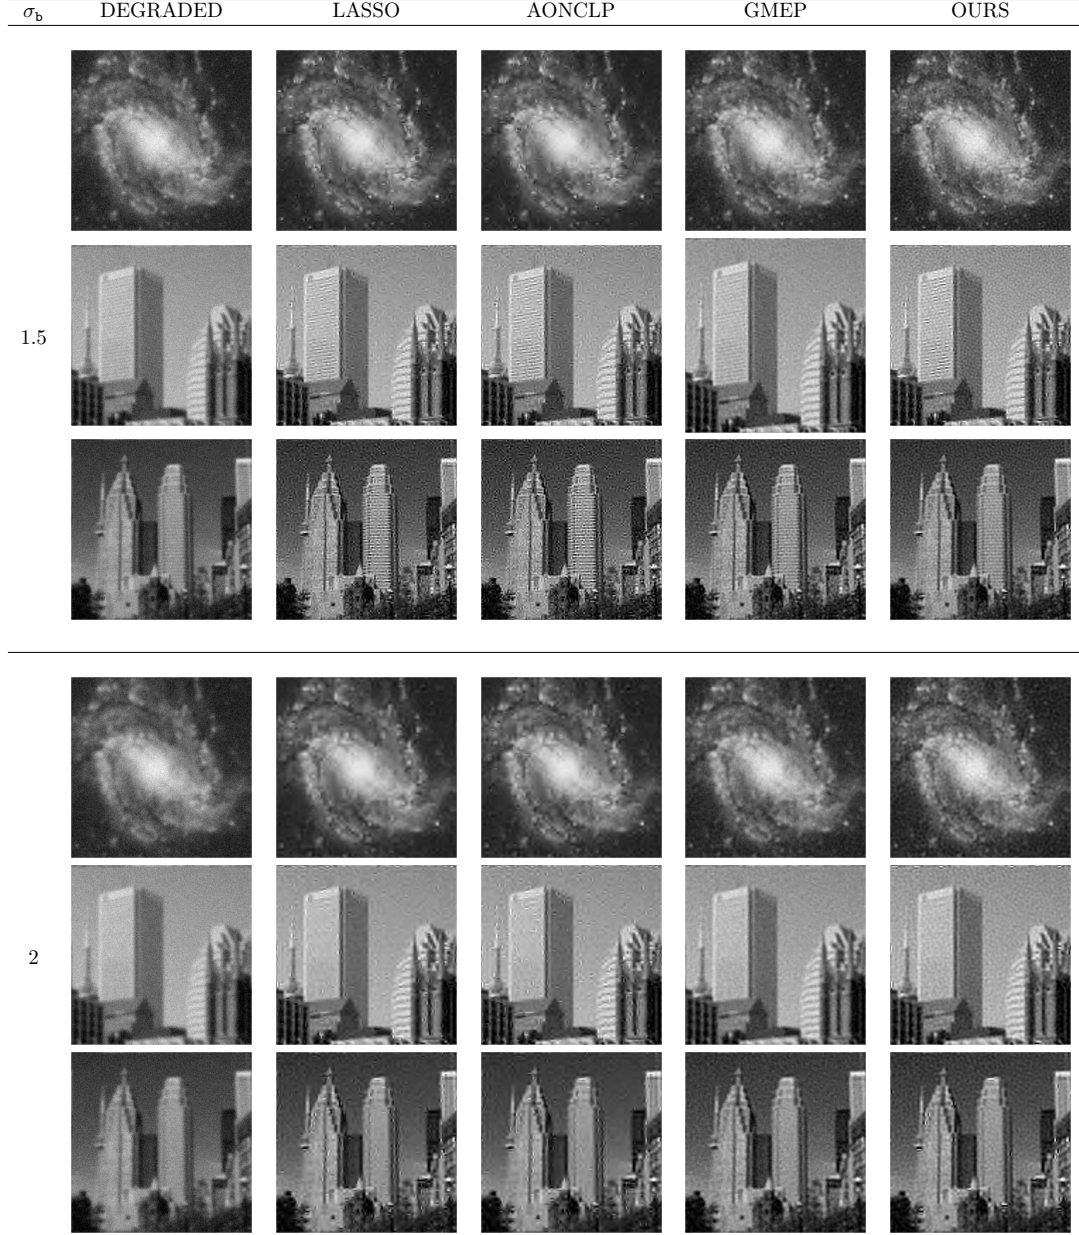  | 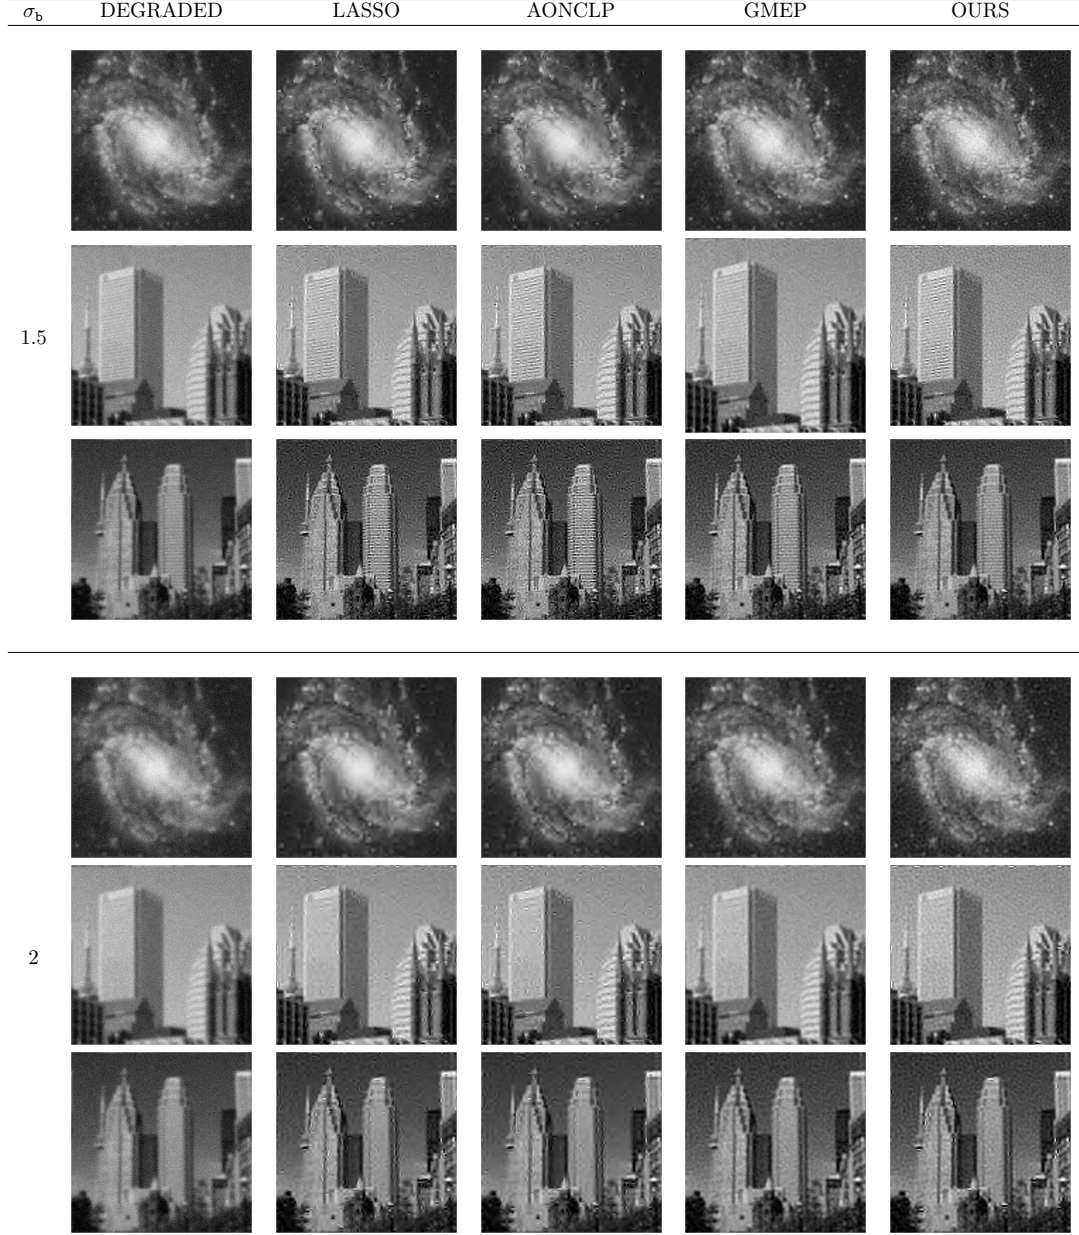  | 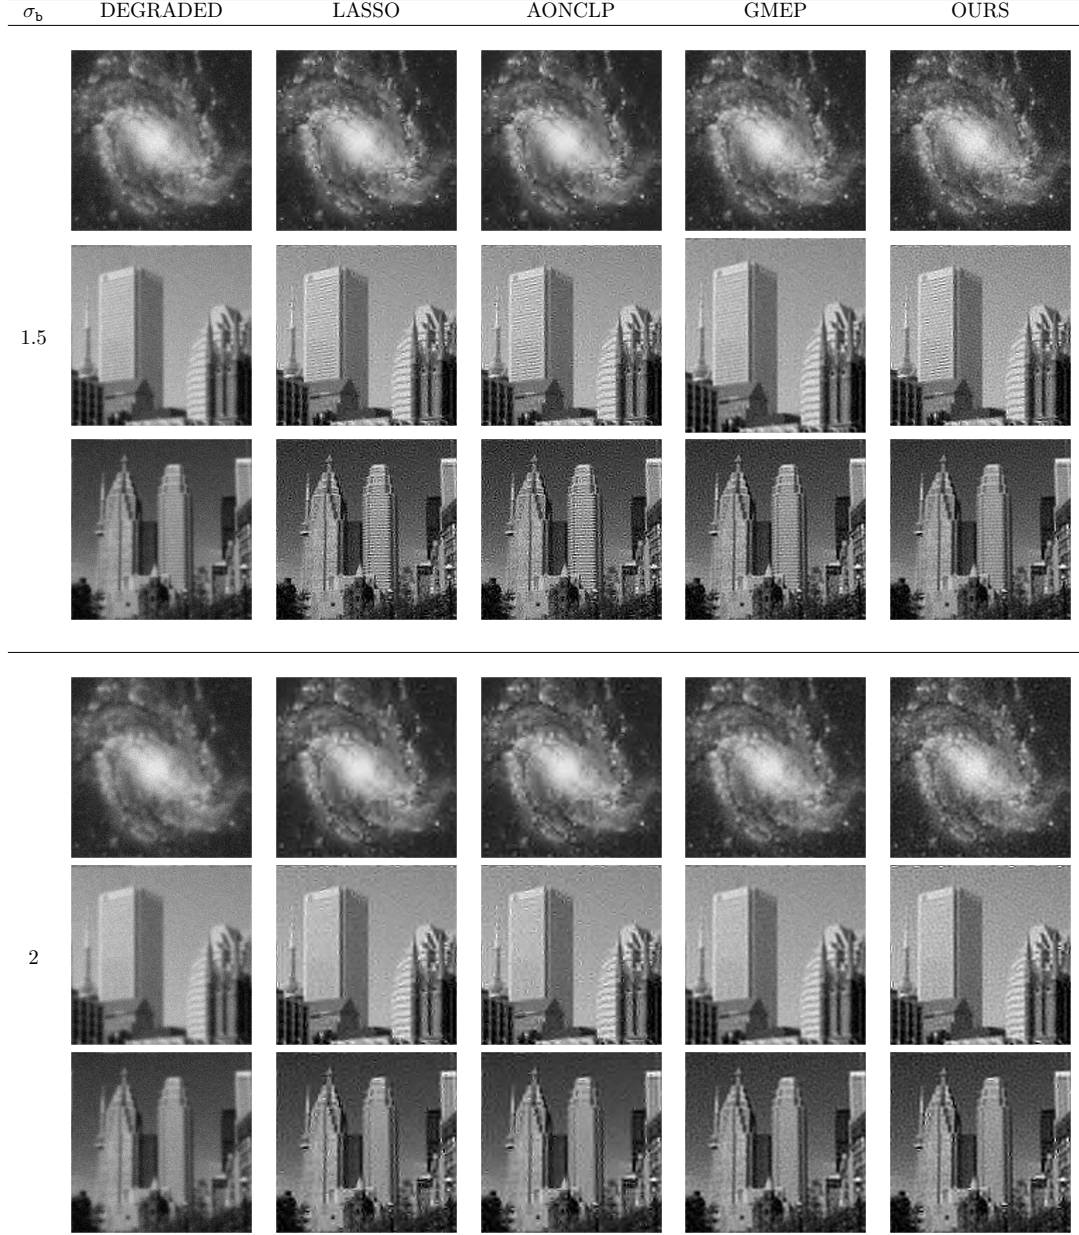  |
|            | 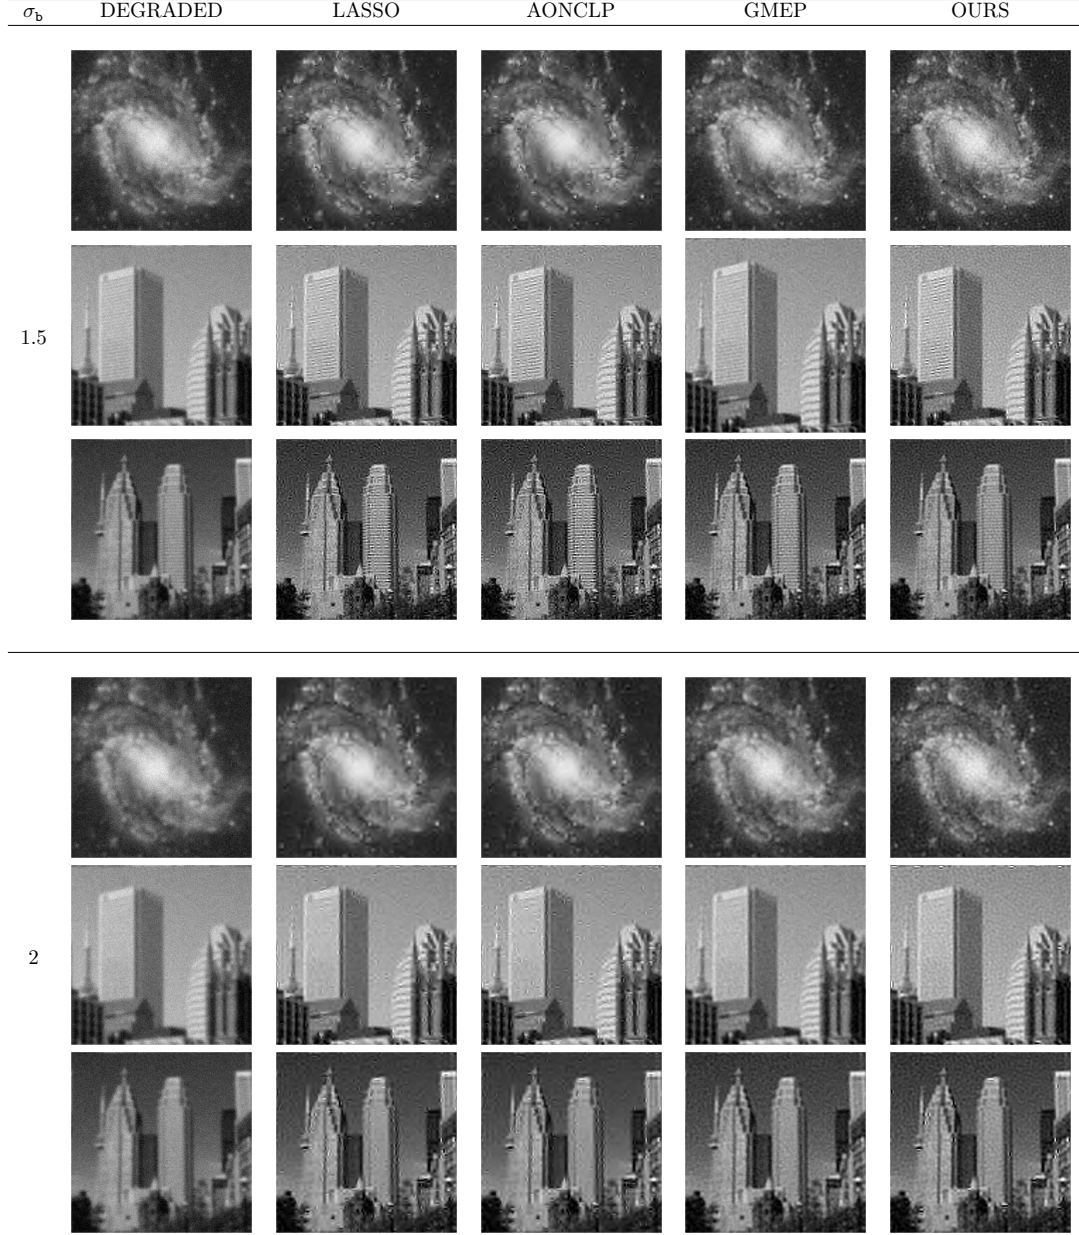 | 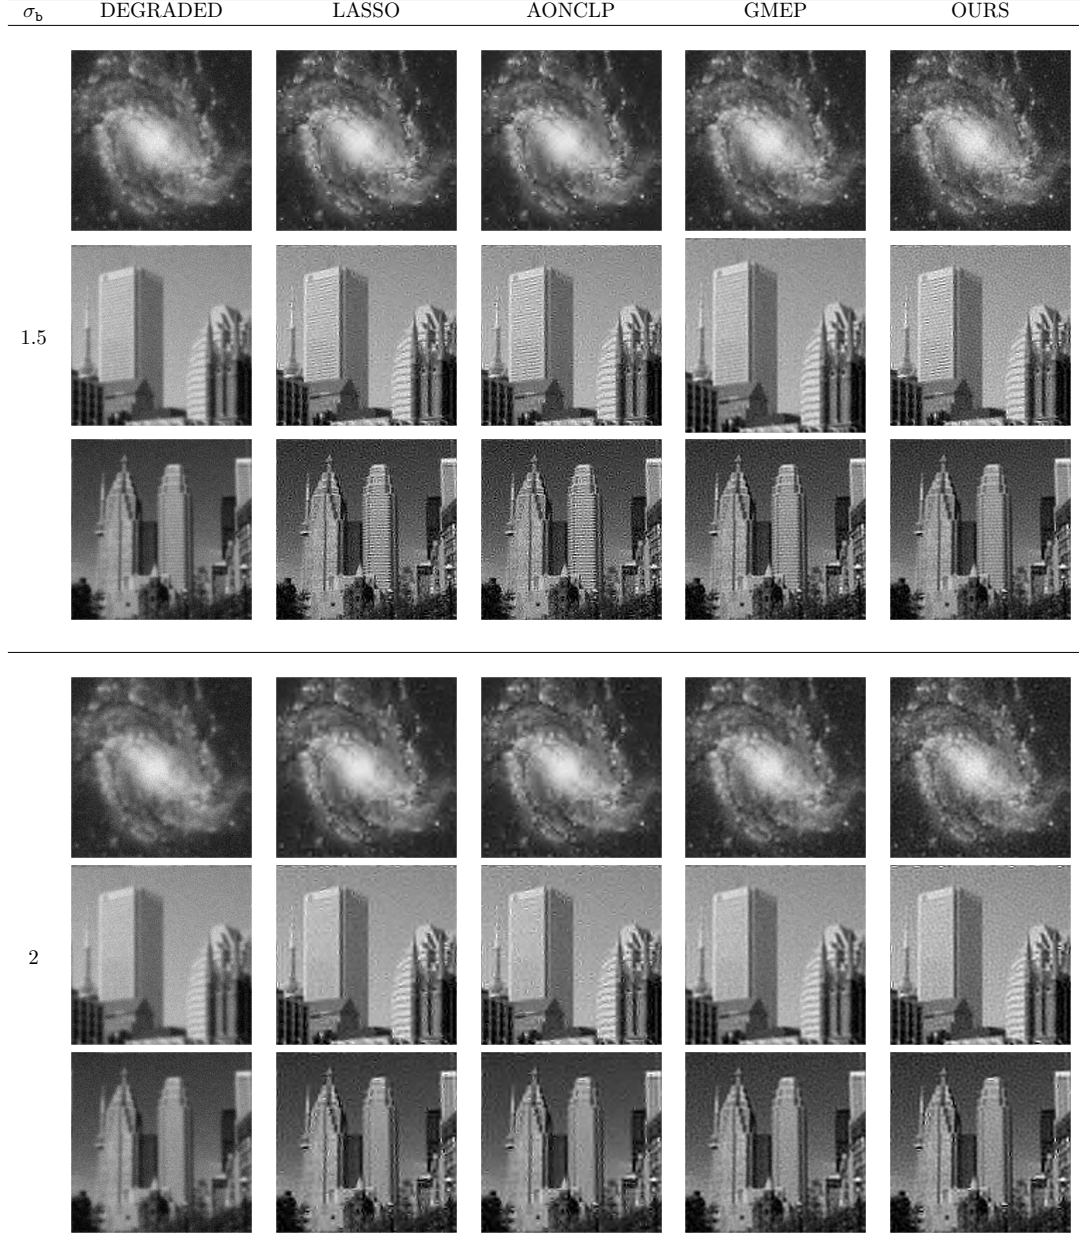 | 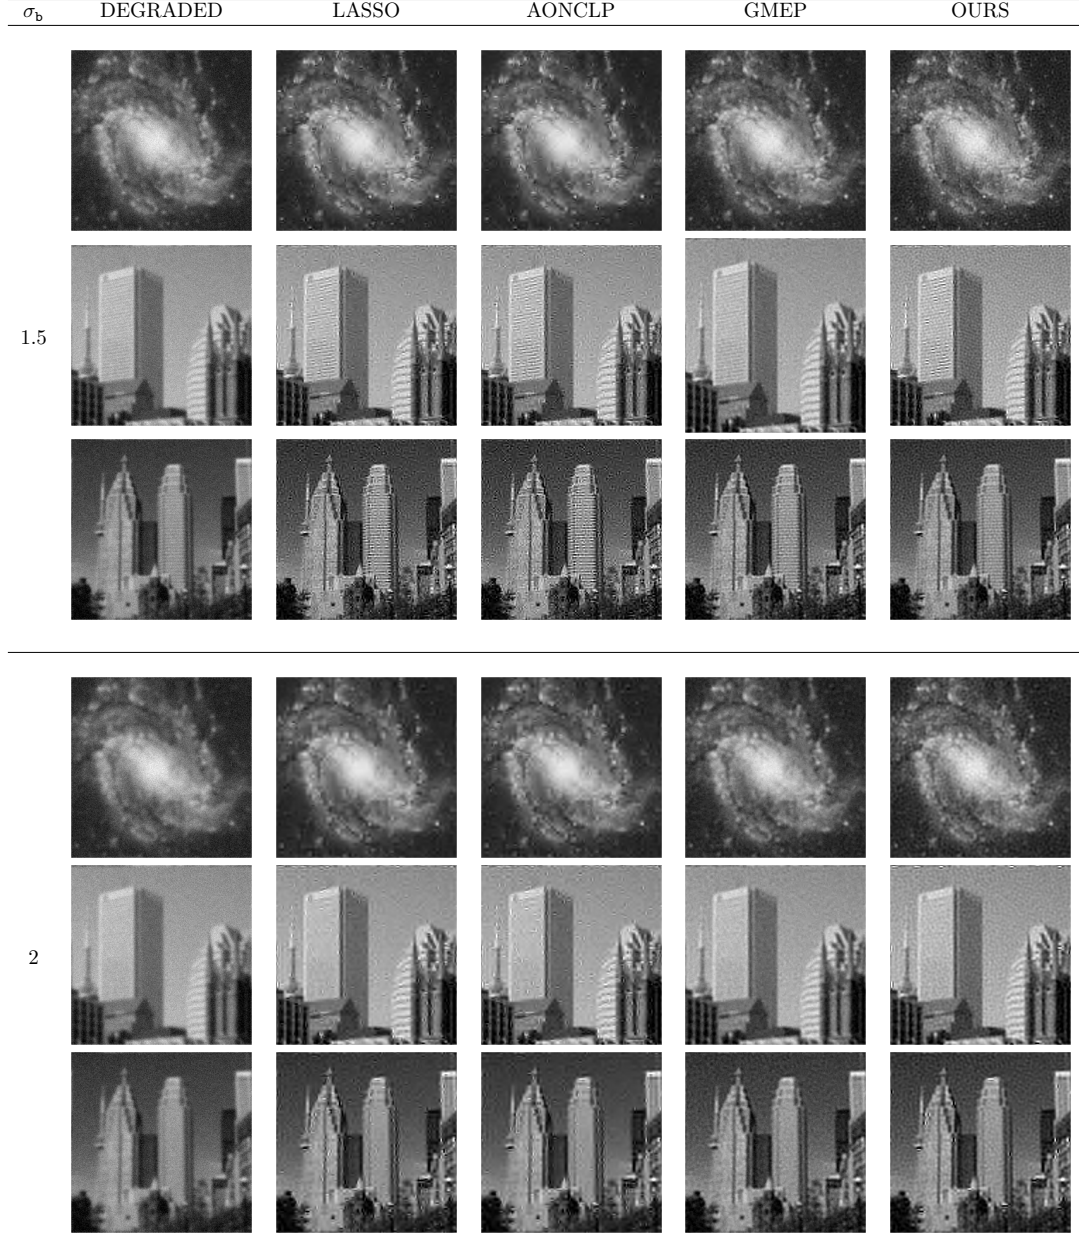 | 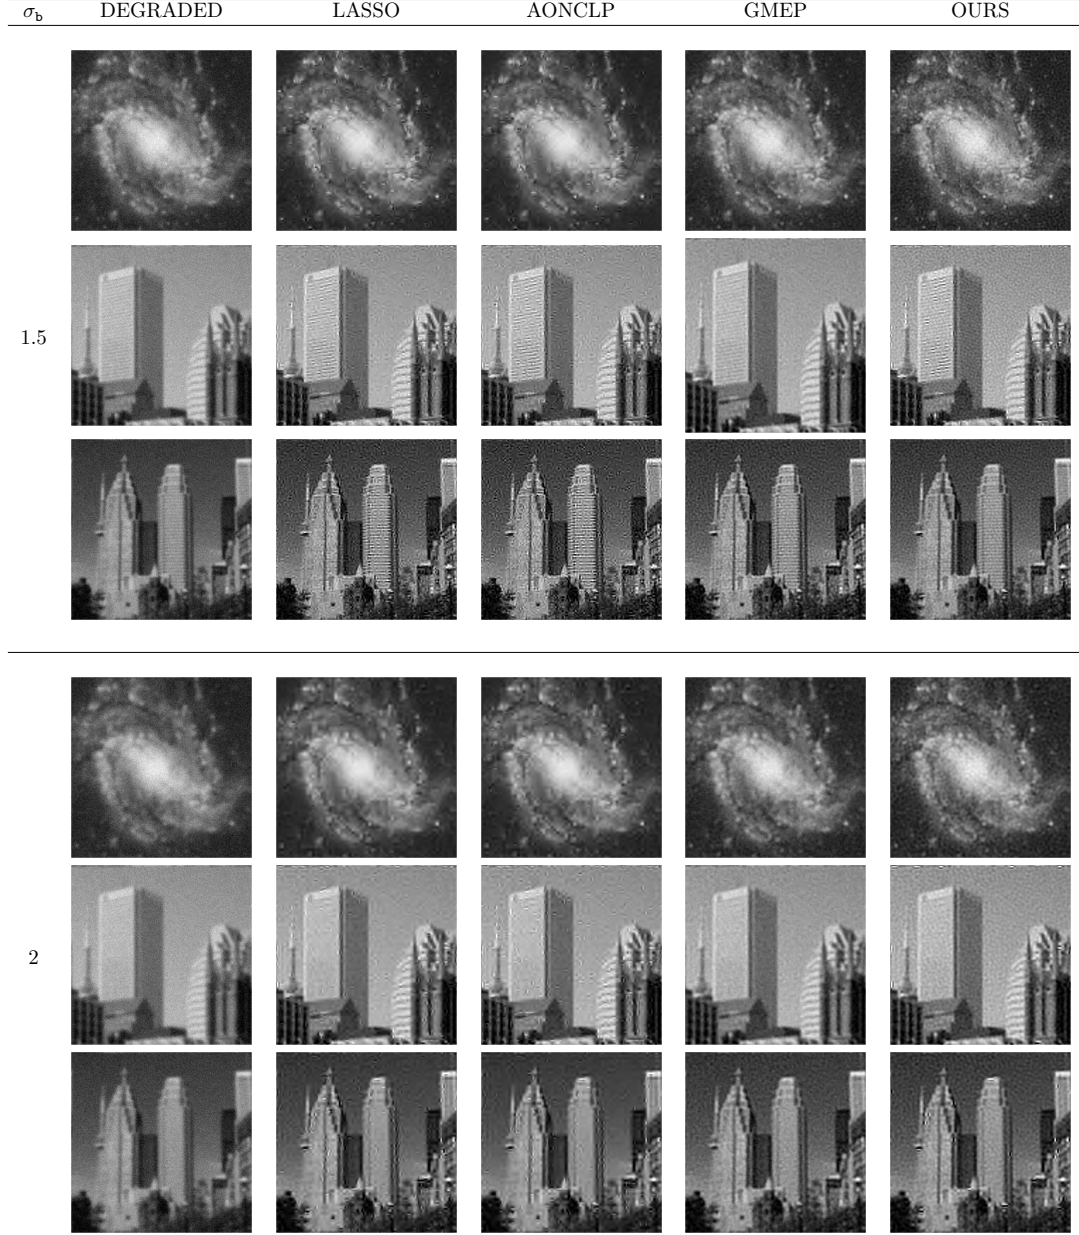 | 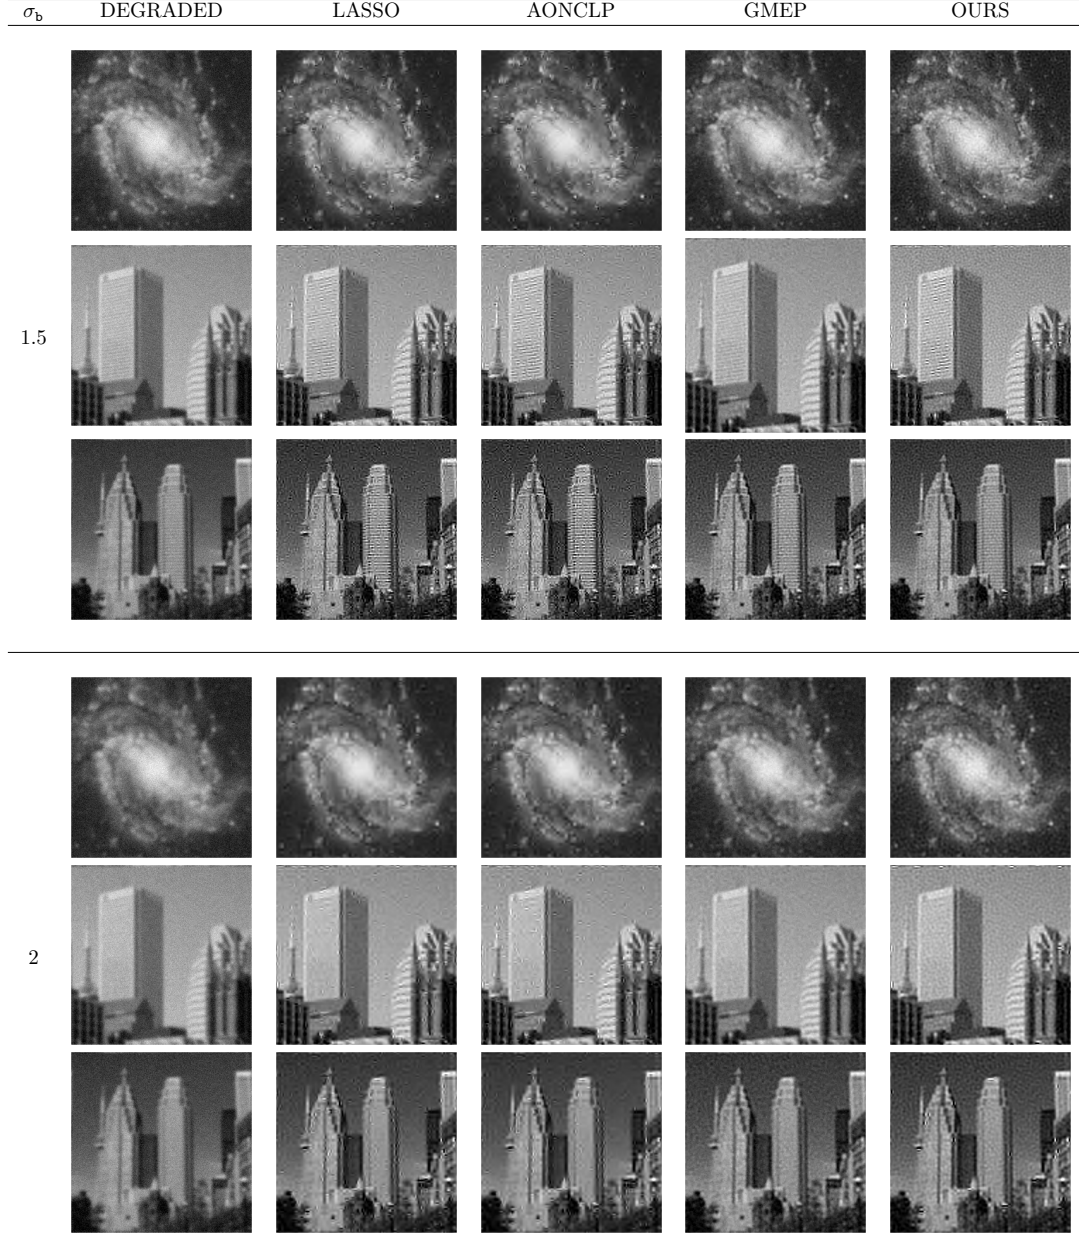 |
|            | 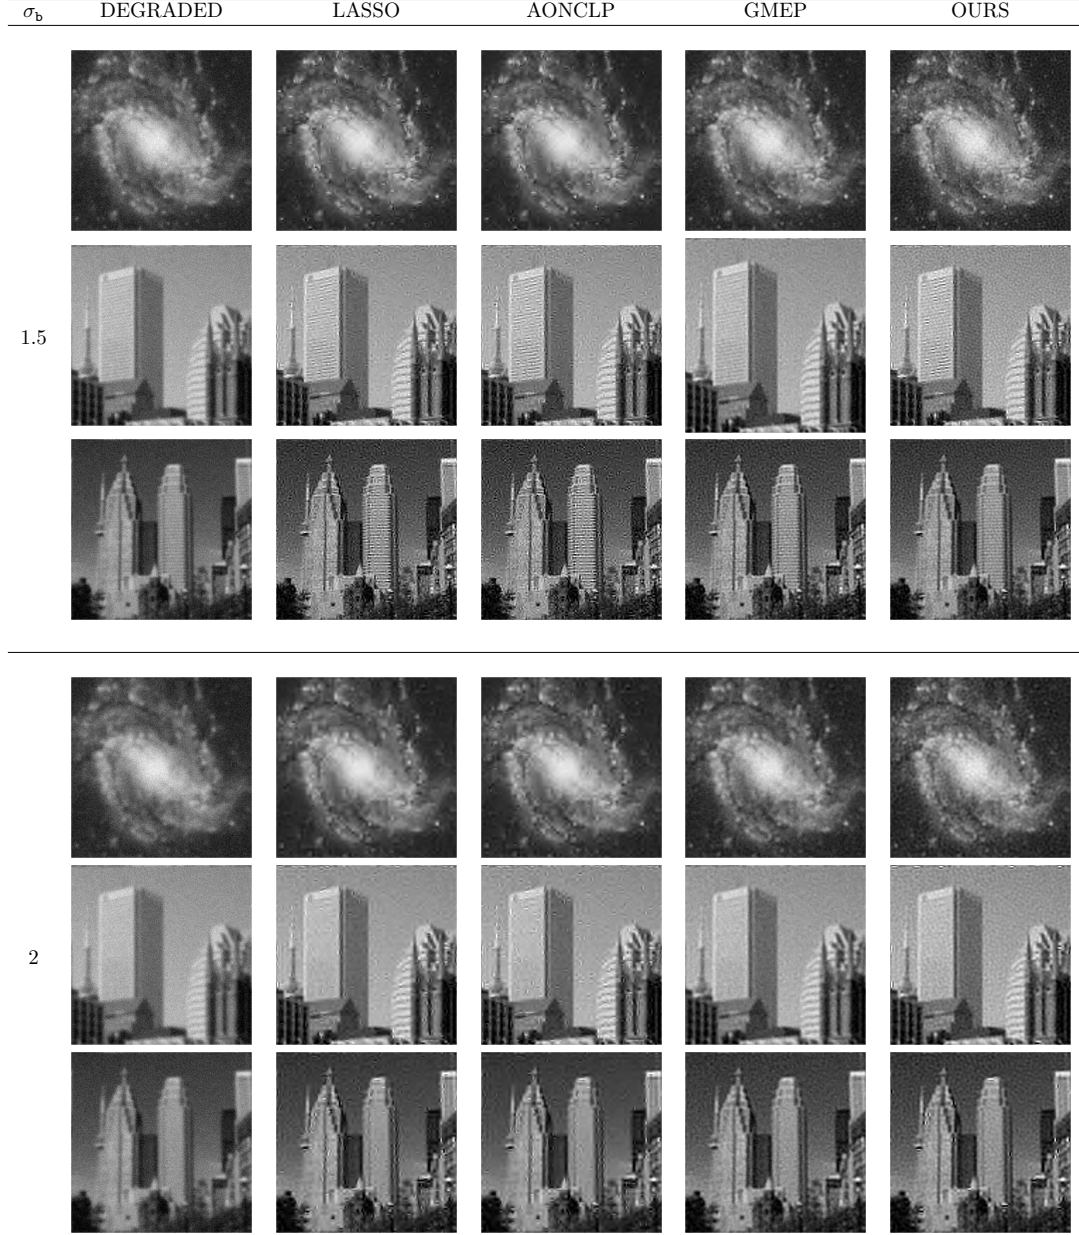 | 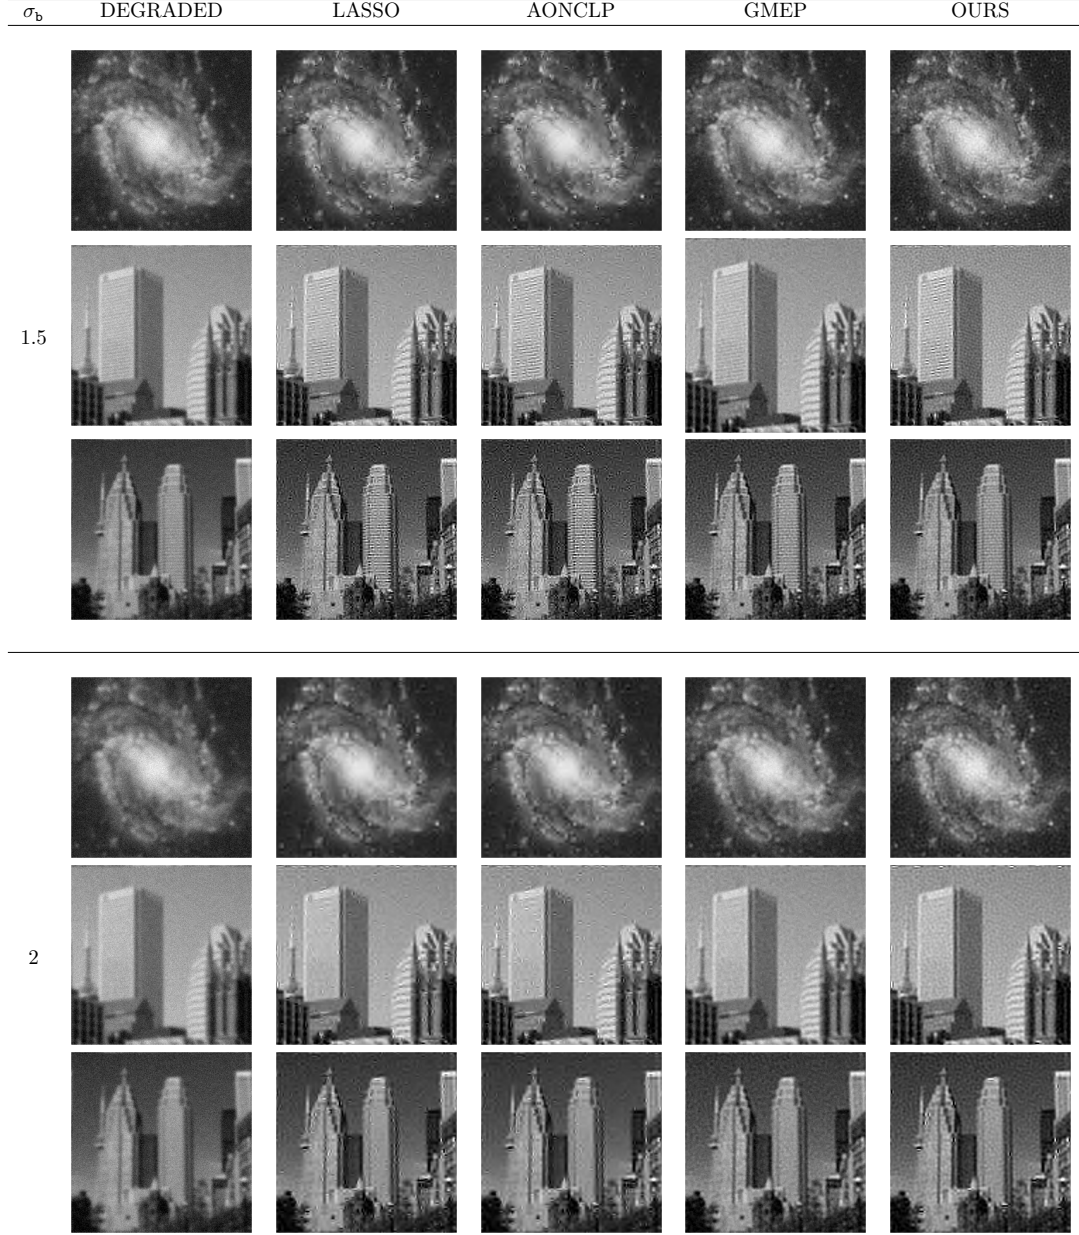 | 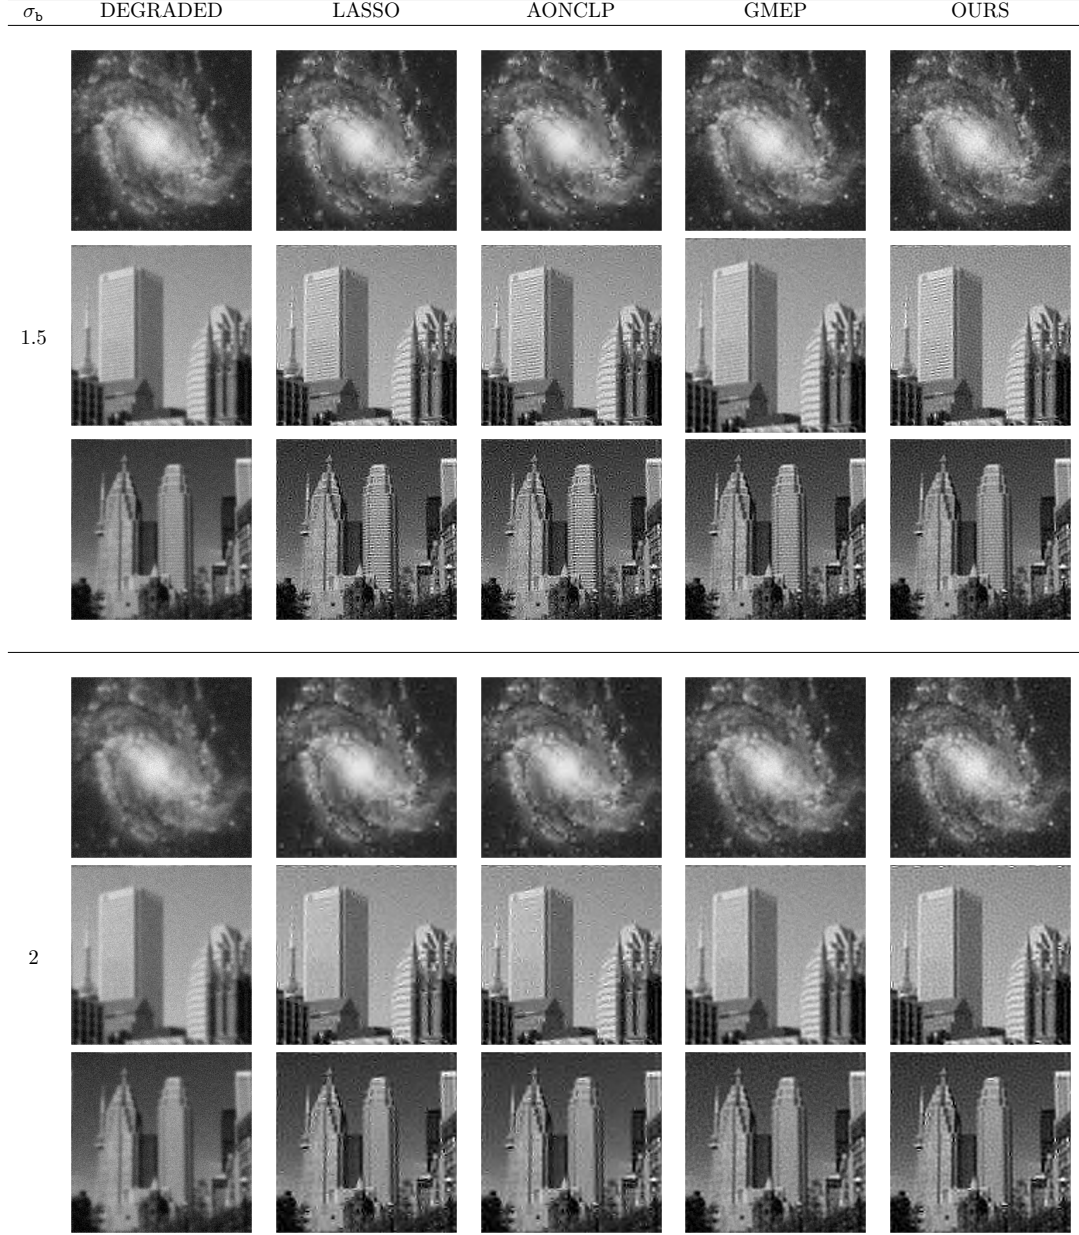 | 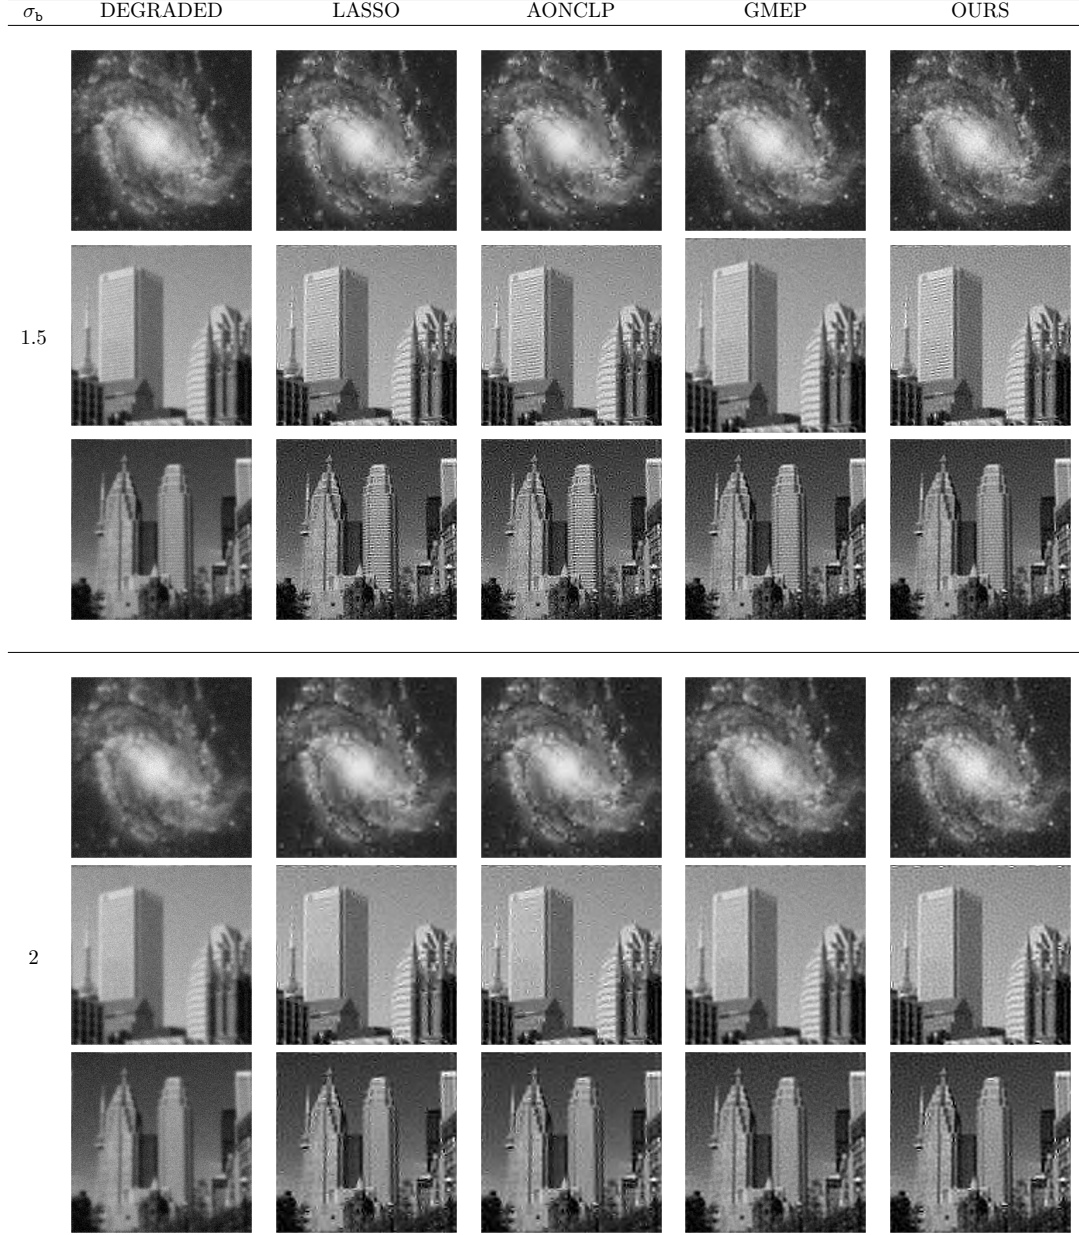 | 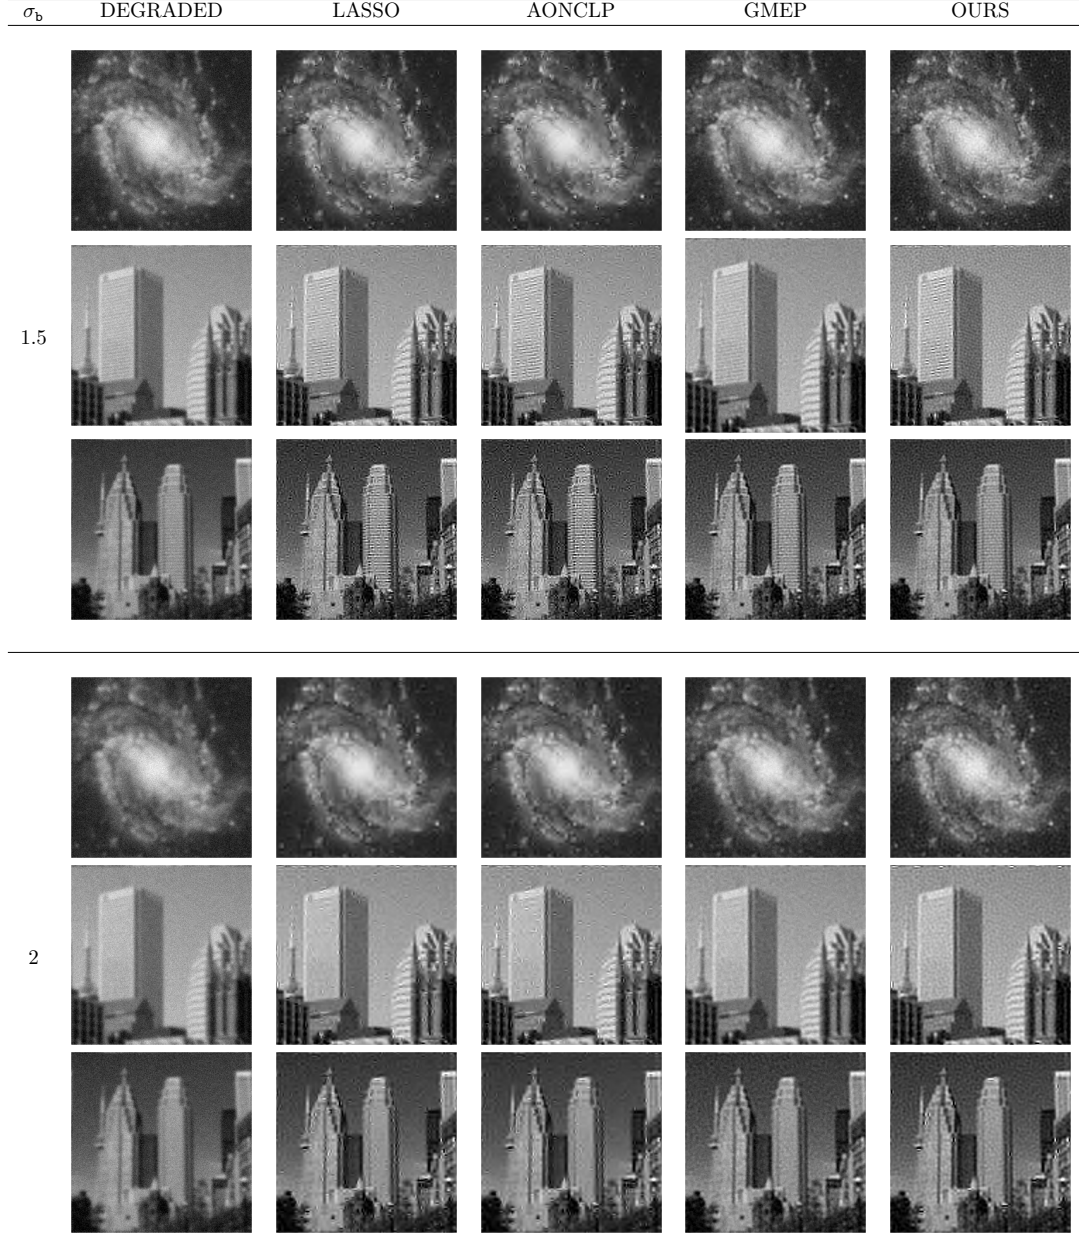 |

**Fig. 8:** Estimated solutions for *Galaxy*, *Buildings* and *Skyscrapers* and  $\sigma = 10$ . First column: Degraded image. Second column: LASSO regularisation. Third column: AONCLP regularisation. Fourth column: GMEP regularisation. Fifth column: Proposed regularisation. First line:  $\sigma_b = 1.5$ , Second line:  $\sigma_b = 2$

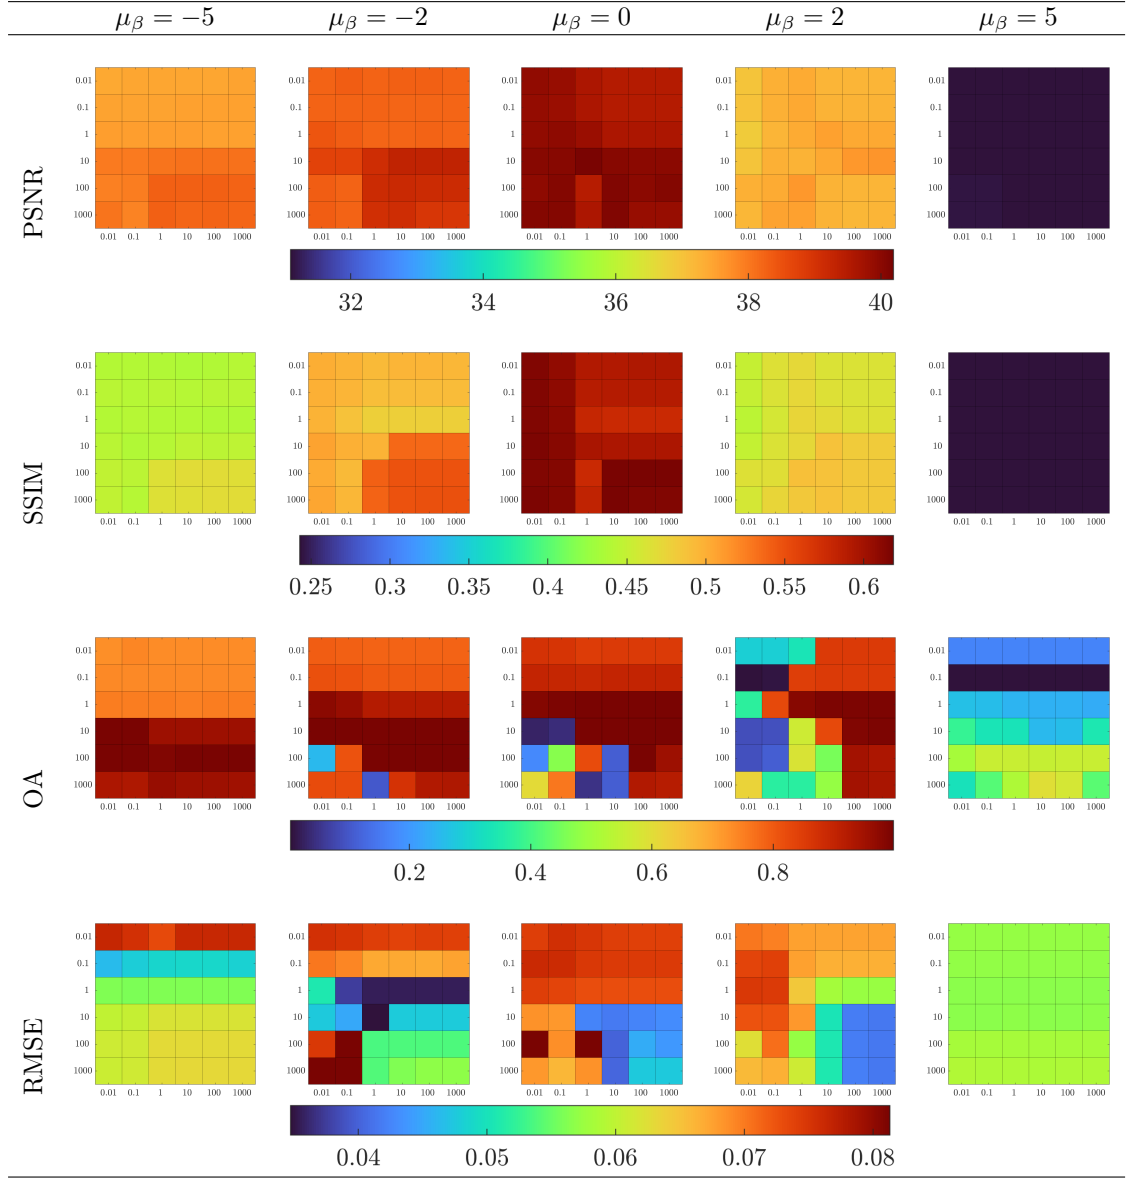

**Fig. 9:** Illustration of the PSNR, SSIM, OA and RMSE values obtained with a grid search on parameters  $(\lambda, \zeta)$  for *Simu1* and 5 different choices for parameter  $\mu_\beta$ . In each matrix, rows correspond to the values for  $\lambda$  and columns to the values for  $\zeta$ . For each parameter we chose 6 values in a logarithmic scale between  $10^{-2}$  and  $10^3$ .

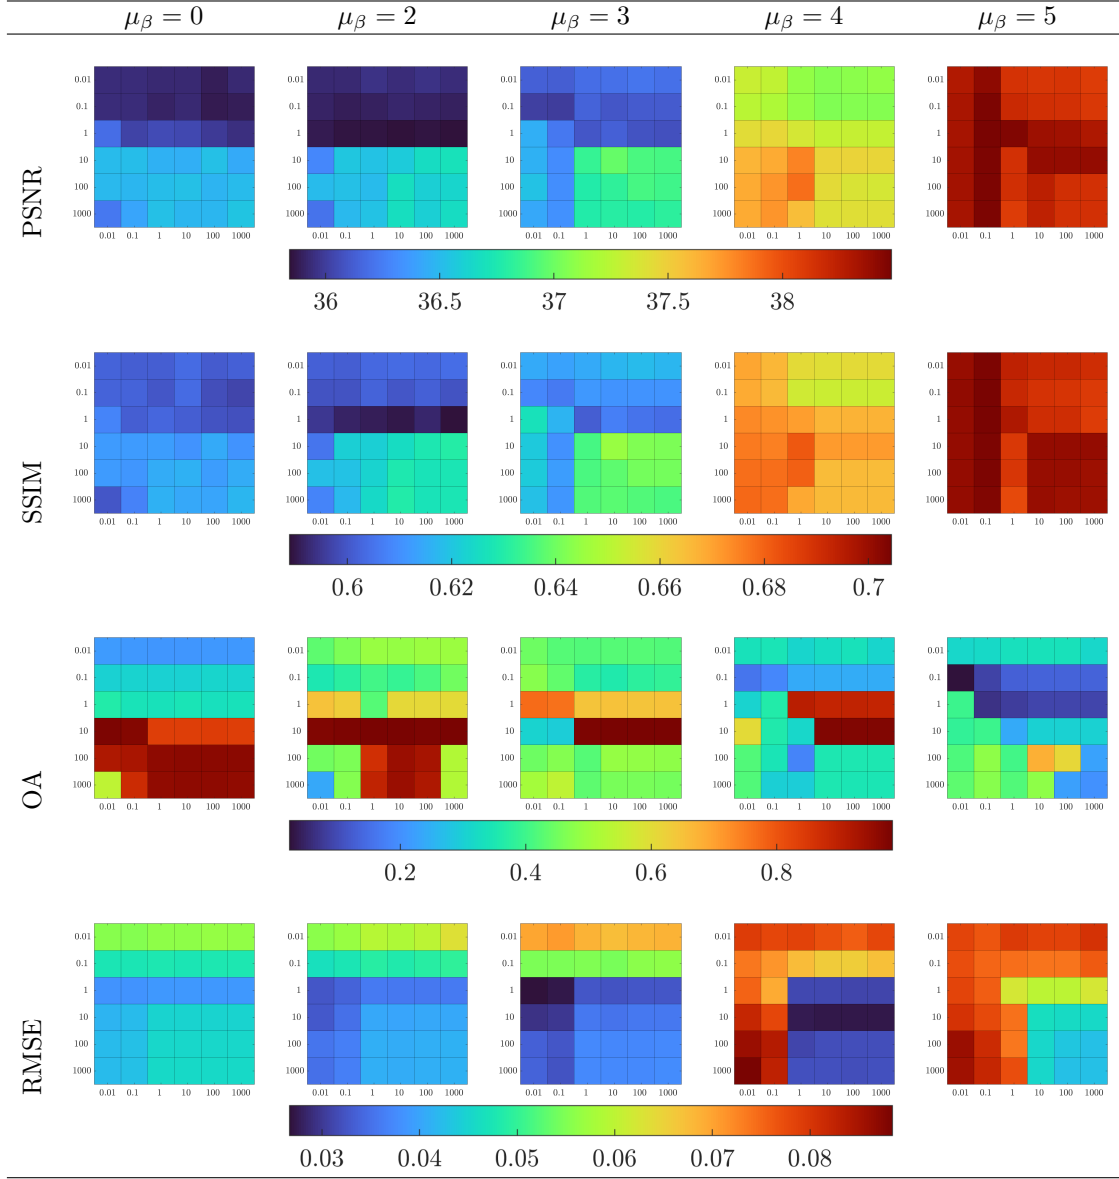

**Fig. 10:** Illustration of the PSNR, SSIM, OA and RMSE values obtained with a grid search on parameters  $(\lambda, \zeta)$  for *Simu2* and 5 different choices for parameter  $\mu_\beta$ . In each matrix, rows correspond to the values for  $\lambda$  and columns to the values for  $\zeta$ . For each parameter we chose 6 values in a logarithmic scale between  $10^{-2}$  and  $10^3$ .

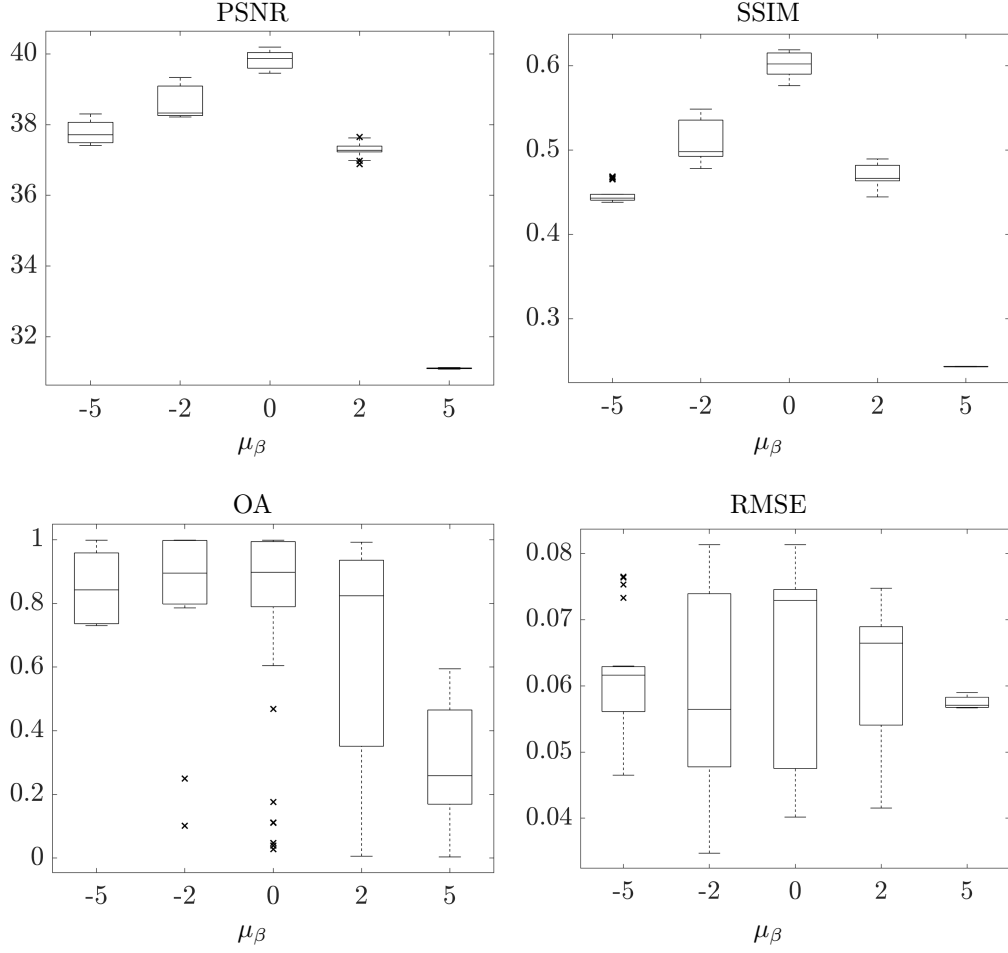

**Fig. 11:** Boxplots of the PSNR, SSIM, OA and RMSE values obtained with a grid search on parameters  $(\lambda, \zeta)$  for *Simu1* and 5 different choices for parameter  $\mu_\beta$ .



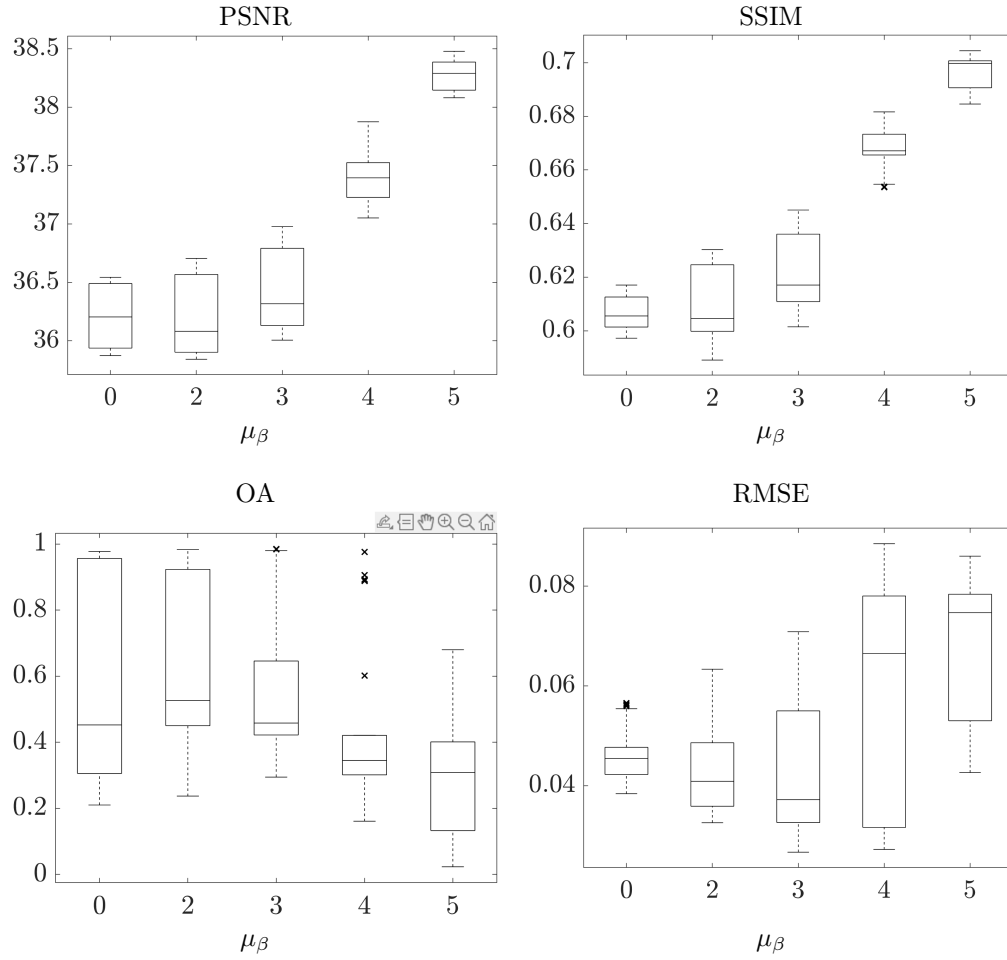

**Fig. 12:** Boxplots of the PSNR, SSIM, OA and RMSE values obtained with a grid search on parameters  $(\lambda, \zeta)$  for *Simu2* and 5 different choices for parameter  $\mu_\beta$ .
